# Supplementary material for: Is it possible to construct asymptotically flat initial data using the evolutionary forms of the constraints?
Source: arXiv:2302.00590 ancillary file (2023-04-11)
Supplement: Supplementary file 1 [file KerrKerrSchild-spinweighted.pdf]

# Spin-weighted variables from a Kerr-Schild time slice of Kerr

This notebook is to construct a Kerr-Schild  $t = \text{const}$  slice of Kerr metric and then derive the spin-weighted variables defined in Rácz and Winicour 2018 Class. Quantum Grav. 35 135002 from this slice.

Instead of the usual Cartesian Kerr-Schild coordinates, here we use the spherical Kerr-Schild coordinates of Chen et al 2021 Phys. Rev. D 104 8 084046. Hereby we warn the reader that the notation conforms to the one used in Rácz and Winicour 2018 Class. Quantum Grav. 35 135002 instead of the one used in Csukás, Rácz 2020 Class. Quantum Grav. 37 155006. This is particularly confusing regarding the secondary shift, where  $\mathbb{N} = q^i \hat{N}_i$  and  $\tilde{\mathbb{N}} = q_i \hat{N}^i$  in the old notation while the use of  $q^i \hat{N}_i$  is avoided in the newer papers and  $\boldsymbol{N} = q_i \hat{N}^i$  (not to confuse with  $\mathbb{N}$ ).

## Coordinate transformation and spin-weighted spherical harmonics utilities

### 4-dimensional metric

In their Kerr-Schild form the metric can be written as

$$g_{ab} = \eta_{ab} + 2 H l_a l_b,$$

where  $\eta_{ab}$  is the Minkowski background and  $l_a$  is a null vector with respect to both  $g_{ab}$  and  $\eta_{ab}$ .

We start with Cartesian coordinates and then apply a coordinate transformation to arrive at spherical Kerr-Schild coordinates.

### Metric in Cartesian coordinates

```
Label Cartesian Kerr-Schild coordinates as (t, x, y, z)

In[8]:= xCA = {t, x, y, z};

Minkowski background

In[9]:= ηCab = {{-1, 0, 0, 0}, {0, 1, 0, 0}, {0, 0, 1, 0}, {0, 0, 0, 1}};

Null vector (see Wiltshire, Visser, Scott The Kerr spacetime eq. (1.32))

In[10]:= lCa = {1, ρ[x, y, z] x + a y, ρ[x, y, z] y - a x, z};

Scalar function H

In[11]:= HCRule = HC → Function[{x, y, z}, M ρ[x, y, z]^3 / (ρ[x, y, z]^4 + a^2 z^2)];

Scalar field ρ as function of coordinates

In[12]:= Solve[ x^2 + y^2 / (ρ[x, y, z]^2 + a^2) + z^2 / ρ[x, y, z]^2 == 1, ρ[x, y, z]]][[4, 1]]
ρCRule = ρ → Function[{x, y, z}, Evaluate[%[2]]];

Out[12]:= ρ[x, y, z] → (sqrt(-a^2 + x^2 + y^2 + z^2) + sqrt(4 a^2 z^2 + (a^2 - x^2 - y^2 - z^2)^2)) / sqrt(2)

Inverse Minkowski (yes it is trivial, but still)

In[14]:= ηCAB = Inverse[ηCab];

The null vector is indeed null

In[15]:= CHECK == Simplify[Sum[ηCAB[[i, j]] * lCa[[i]] * lCa[[j]], {i, 1, 4}, {j, 1, 4}] /. ρCRule]
Out[15]:= CHECK == 0

In[16]:= lCA = Table[Sum[ηCAB[[i, ii]] * lCa[[ii]], {ii, 1, 4}], {i, 1, 4}];

Physical metric g_ab

In[17]:= gCab = Table[ηCab[[i, j]] + 2 HC[x, y, z] * lCa[[i]] * lCa[[j]], {i, 1, 4}, {j, 1, 4}];

In[18]:= gCAB = Inverse[gCab];

Check the formula for the inverse metric

In[19]:= CHECK == MatrixForm[Simplify[Table[gCAB[[i, j]] - (ηCAB[[i, j]] - 2 HC[x, y, z] * lCa[[i]] * lCa[[j]]) /. ρCRule, {i, 1, 4}, {j, 1, 4}]]]
Out[19]:= CHECK == (0 0 0 0; 0 0 0 0; 0 0 0 0; 0 0 0 0)
```

# Transform to spherical Kerr-Schild coordinates

The coordinate transformation applied here is a composition of the described by Chen et al

$$\frac{\bar{x}}{\rho} = \frac{x}{\sqrt{\rho^2+a^2}}$$

$$\frac{\bar{y}}{\rho} = \frac{y}{\sqrt{\rho^2+a^2}}$$

$$\bar{z} = z$$

and a transformation into standard spherical coordinates

$$\bar{x} = r \sin\vartheta \cos\varphi$$

$$\bar{y} = r \sin\vartheta \sin\varphi$$

$$\bar{z} = r \cos\vartheta$$

with  $r = \rho$ . The new coordinates are labelled by  $(t, r, \vartheta, \varphi)$ .

```
In[20]:= xA = {t, r, \vartheta, \varphi};
```

The composition gives

$$x = \sqrt{r^2+a^2} \sin\vartheta \cos\varphi$$

$$y = \sqrt{r^2+a^2} \sin\vartheta \sin\varphi$$

$$z = r \cos\vartheta.$$

```
In[21]:= tr = {t, \sqrt{r^2+a^2} Sin[\vartheta] Cos[\varphi], \sqrt{r^2+a^2} Sin[\vartheta] Sin[\varphi], r Cos[\vartheta]};
```

```
In[22]:= Jac = Jacobi[tr, xA];
MatrixForm[Jac]
```

Out[23]/MatrixForm=

$$\begin{pmatrix} 1 & 0 & 0 & 0 \\ 0 & \frac{r \cos[\varphi] \sin[\vartheta]}{\sqrt{a^2+r^2}} & \sqrt{a^2+r^2} \cos[\vartheta] \cos[\varphi] & -\sqrt{a^2+r^2} \sin[\vartheta] \sin[\varphi] \\ 0 & \frac{r \sin[\varphi] \sin[\vartheta]}{\sqrt{a^2+r^2}} & \sqrt{a^2+r^2} \cos[\vartheta] \sin[\varphi] & \sqrt{a^2+r^2} \cos[\varphi] \sin[\vartheta] \\ 0 & \cos[\vartheta] & -r \sin[\vartheta] & 0 \end{pmatrix}$$

Recognize the spherical metric when  $a \rightarrow 0$

```
In[24]:= \eta_{ab} = TFMat[\eta_{Cab}, Jac] // Simplify;
MatrixForm[%]
% /. a -> 0
```

Out[25]/MatrixForm=

$$\begin{pmatrix} -1 & 0 & 0 & 0 \\ 0 & \frac{a^2+2 r^2+a^2 \cos[2 \vartheta]}{2 (a^2+r^2)} & 0 & 0 \\ 0 & 0 & \frac{1}{2} (a^2+2 r^2+a^2 \cos[2 \vartheta]) & 0 \\ 0 & 0 & 0 & (a^2+r^2) \sin[\vartheta]^2 \end{pmatrix}$$

Out[26]=  $\{-1, 0, 0, 0\}, \{0, 1, 0, 0\}, \{0, 0, r^2, 0\}, \{0, 0, 0, r^2 \sin[\vartheta]^2\}$

```
In[27]:= \eta_{AB} = Inverse[\eta_{ab}] // Simplify;
MatrixForm[%]
```

Out[28]/MatrixForm=

$$\begin{pmatrix} -1 & 0 & 0 & 0 \\ 0 & \frac{2 (a^2+r^2)}{a^2+2 r^2+a^2 \cos[2 \vartheta]} & 0 & 0 \\ 0 & 0 & \frac{2}{a^2+2 r^2+a^2 \cos[2 \vartheta]} & 0 \\ 0 & 0 & 0 & \frac{\csc[\vartheta]^2}{a^2+r^2} \end{pmatrix}$$

The components of null vector  $l$

```
In[29]:= l_a = TFVec[l_Ca, Jac] /. \rho[x, y, z] -> r /. xCA[[2]] -> tr[[2]] /. xCA[[3]] -> tr[[3]] /. xCA[[4]] -> tr[[4]] // Simplify
```

Out[29]=  $\left\{1, \frac{a^2+2 r^2+a^2 \cos[2 \vartheta]}{2 (a^2+r^2)}, 0, -a \sin[\vartheta]^2\right\}$

```
In[30]:= l_A = Table[Sum[\eta_{AB}[[i, j]] \times l_a[[j]], {j, 1, 4}], {i, 1, 4}]
```

Out[30]=  $\left\{-1, 1, 0, -\frac{a}{a^2+r^2}\right\}$

```
In[31]:= CHECK == Sum[l_A[[i, j]] \times l_a[[j]], {j, 1, 4}] // Simplify
```

Out[31]= CHECK == 0

```
In[32]:= HC[x, y, z] /. HCRule /. \rho[x, y, z] -> r /. xCA[[2]] -> tr[[2]] /. xCA[[3]] -> tr[[3]] /. xCA[[4]] -> tr[[4]] // Simplify
HRule = H -> Function[{r, \vartheta}, Evaluate[%]];
M r
```

Out[32]=  $\frac{M r}{r^2+a^2 \cos[\vartheta]^2}$

Constructing the physical metric in spherical coordinates

```
In[34]:= gab = Table[ηab[[i, j]] + 2 H[r, ϑ] × /a[[i]] × /a[[j]], {i, 1, 4}, {j, 1, 4}] /. HRule // Simplify ;
MatrixForm[%]
```

Out[35]//MatrixForm=

$$\begin{pmatrix} -1 + \frac{2 M r}{r^2 + a^2 \cos^2[\vartheta]} & \frac{2 M r}{a^2 + r^2} & 0 & -\frac{2 a M r \sin[\vartheta]^2}{r^2 + a^2 \cos^2[\vartheta]} \\ \frac{2 M r}{a^2 + r^2} & \frac{(a^2 + r^2 (2 M + r)) (a^2 + 2 r^2 + a^2 \cos[2 \vartheta])}{2 (a^2 + r^2)^2} & 0 & -\frac{2 a M r \sin[\vartheta]^2}{a^2 + r^2} \\ 0 & 0 & \frac{1}{2} (a^2 + 2 r^2 + a^2 \cos[2 \vartheta]) & 0 \\ -\frac{2 a M r \sin[\vartheta]^2}{r^2 + a^2 \cos^2[\vartheta]} & -\frac{2 a M r \sin[\vartheta]^2}{a^2 + r^2} & 0 & \sin[\vartheta]^2 \left( a^2 + r^2 + \frac{2 a^2 M r \sin[\vartheta]^2}{r^2 + a^2 \cos^2[\vartheta]} \right) \end{pmatrix}$$

Reintroducing H(r,ϑ)

$$\text{In[36]:= } \mathbf{gabH} = \begin{pmatrix} -1 + 2 H[r, \vartheta] & \frac{2 M r}{a^2 + r^2} & 0 & -2 a H[r, \vartheta] \sin[\vartheta]^2 \\ \frac{2 M r}{a^2 + r^2} & \frac{(r^2 + a^2 \cos^2[\vartheta]) (a^2 + r^2 + 2 M r)}{(a^2 + r^2)^2} & 0 & -\frac{a 2 M r \sin[\vartheta]^2}{a^2 + r^2} \\ 0 & 0 & r^2 + a^2 \cos^2[\vartheta] & 0 \\ -2 a H[r, \vartheta] \sin[\vartheta]^2 & -\frac{a 2 M r \sin[\vartheta]^2}{a^2 + r^2} & 0 & \sin[\vartheta]^2 (a^2 + r^2 + 2 a^2 H[r, \vartheta] \sin[\vartheta]^2) \end{pmatrix};$$

CHECK == gabH - gab /. HRule // Simplify

Out[37]= CHECK == {{0, 0, 0, 0}, {0, 0, 0, 0}, {0, 0, 0, 0}, {0, 0, 0, 0}}

Inverse metric

```
In[38]:= gAB = Table[ηAB[[i, j]] - 2 H[r, ϑ] × /A[[i]] × /A[[j]], {i, 1, 4}, {j, 1, 4}] /. HRule // Simplify ;
MatrixForm[%]
```

Out[39]//MatrixForm=

$$\begin{pmatrix} -1 - \frac{2 M r}{r^2 + a^2 \cos^2[\vartheta]} & \frac{2 M r}{r^2 + a^2 \cos^2[\vartheta]} & 0 & -\frac{2 a M r}{(a^2 + r^2) (r^2 + a^2 \cos^2[\vartheta])} \\ \frac{2 M r}{r^2 + a^2 \cos^2[\vartheta]} & \frac{2 (a^2 + r^2 (-2 M + r))}{a^2 + 2 r^2 + a^2 \cos[2 \vartheta]} & 0 & \frac{2 a M r}{(a^2 + r^2) (r^2 + a^2 \cos^2[\vartheta])} \\ 0 & 0 & \frac{2}{a^2 + 2 r^2 + a^2 \cos[2 \vartheta]} & 0 \\ -\frac{2 a M r}{(a^2 + r^2) (r^2 + a^2 \cos^2[\vartheta])} & \frac{2 a M r}{(a^2 + r^2) (r^2 + a^2 \cos^2[\vartheta])} & 0 & \frac{-\frac{2 a^2 M r}{r^2 + a^2 \cos^2[\vartheta]} + (a^2 + r^2) \csc[\vartheta]^2}{(a^2 + r^2)^2} \end{pmatrix}$$

$$\text{In[40]:= } \mathbf{gABH} = \begin{pmatrix} -1 - 2 H[r, \vartheta] & 2 H[r, \vartheta] & 0 & -\frac{2 a H[r, \vartheta]}{(a^2 + r^2)} \\ 2 H[r, \vartheta] & \left( \frac{a^2 + r^2}{M r} - 2 \right) H[r, \vartheta] & 0 & \frac{2 a H[r, \vartheta]}{(a^2 + r^2)} \\ 0 & 0 & \frac{H[r, \vartheta]}{M r} & 0 \\ -\frac{2 a H[r, \vartheta]}{(a^2 + r^2)} & \frac{2 a H[r, \vartheta]}{(a^2 + r^2)} & 0 & \frac{-2 a^2 H[r, \vartheta] + (a^2 + r^2) \csc[\vartheta]^2}{(a^2 + r^2)^2} \end{pmatrix};$$

CHECK == gABH - gAB /. HRule // Simplify

Out[41]= CHECK == {{0, 0, 0, 0}, {0, 0, 0, 0}, {0, 0, 0, 0}, {0, 0, 0, 0}}

```
In[42]:= gAb = FullSimplify[Table[Sum[gAB[[i, ii]] × gab[[ii, j]], {ii, 1, 4}], {i, 1, 4}, {j, 1, 4}];
CHECK == MatrixForm[Table[gAb[[i, j]] - KroneckerDelta[i, j], {i, 1, 4}, {j, 1, 4}]]
```

$$\text{Out[43]= } \text{CHECK} = \begin{pmatrix} 0 & 0 & 0 & 0 \\ 0 & 0 & 0 & 0 \\ 0 & 0 & 0 & 0 \\ 0 & 0 & 0 & 0 \end{pmatrix}$$

Christoffel symbol

```
In[44]:= ΓAbc = Table[1/2 Sum[gAB[[i, ii]] × (D[gab[[j, ii]], xA[[k]] + D[gab[[k, ii]], xA[[j]] - D[gab[[k, j]], xA[[ii]]]), {ii, 1, 4}], {i, 1, 4}, {j, 1, 4}, {k, 1, 4}];
```

```
In[45]:= ΓAbcH =
Table[1/2 Sum[gABH[[i, ii]] × (D[gabH[[j, ii]], xA[[k]] + D[gabH[[k, ii]], xA[[j]] - D[gabH[[k, j]], xA[[ii]]]), {ii, 1, 4}], {i, 1, 4}, {j, 1, 4}, {k, 1, 4}];
```

Riemann tensor

```
In[46]:= Rabcd = Table[-D[ΓAbc[[l, j, k]], xA[[i]] + D[ΓAbc[[l, i, k]], xA[[j]] +
Sum[-ΓAbc[[l, i, ii]] × ΓAbc[[ii, j, k]] + ΓAbc[[l, j, ii]] × ΓAbc[[ii, i, k]], {ii, 1, 4}], {i, 1, 4}, {j, 1, 4}, {k, 1, 4}, {l, 1, 4}];
```

Checking Ricci flatness

```
In[47]:= Rab = Table[Sum[Rabcd[[i, ii, j, ii]], {ii, 1, 4}], {i, 1, 4}, {j, 1, 4}];
```

```
In[48]:= CHECK == Rab // Simplify
```

Out[48]= CHECK == {{0, 0, 0, 0}, {0, 0, 0, 0}, {0, 0, 0, 0}, {0, 0, 0, 0}}

## 3+1 decomposition

In this section we consider  $t = \text{const}$  hypersurfaces and decompose the metric to parallel and transverse components.

■ Computing induced metric

The normal 1-form is  $(dt)_a$

```
In[49]:= dTa = {1, 0, 0, 0};

In[50]:= dTA = Table[Sum[gAB[[i, ii]] * dTa[[ii]], {ii, 1, 4}], {i, 1, 4}]

Out[50]:= {-1 - (2 M r)/(r^2 + a^2 Cos[ø]^2), (2 M r)/(r^2 + a^2 Cos[ø]^2), 0, -(2 a M r)/((a^2 + r^2) (r^2 + a^2 Cos[ø]^2))}
```

The unit normal is then  $(dt)_a/N$  with  $N = \sqrt{-g^{ab}(dt)_a (dt)_b}$

```
In[51]:= na = -dTa / Sqrt[-Sum[gAB[[i, j]] * dTa[[i]] * dTa[[j]], {i, 1, 4}, {j, 1, 4}]]

Out[51]:= {-1/Sqrt[1 + (2 M r)/(r^2 + a^2 Cos[ø]^2)], 0, 0, 0}
```

$naH = -dTa / Sqrt[-Sum[gABH[[i, j]] * dTa[[i]] * dTa[[j]], {i, 1, 4}, {j, 1, 4}]]$

```
Out[52]:= {-1/Sqrt[1 + 2 H[r, ø]], 0, 0, 0}
```

$na = Table[Sum[gAB[[i, ii]] * na[[ii]], {ii, 1, 4}], {i, 1, 4}] // Simplify$

```
Out[53]:= {Sqrt[1 + (2 M r)/(r^2 + a^2 Cos[ø]^2)], -(2 M r)/((r^2 + a^2 Cos[ø]^2) Sqrt[1 + (2 M r)/(r^2 + a^2 Cos[ø]^2)]), 0, (2 a M r)/((a^2 + r^2) (r^2 + a^2 Cos[ø]^2) Sqrt[1 + (2 M r)/(r^2 + a^2 Cos[ø]^2)])}
```

Check the unit norm

```
In[54]:= CHECK == Sum[na[[ii]] * na[[ii]], {ii, 1, 4}] - (-1) // Simplify

Out[54]:= CHECK == 0
```

Induced inverse metric  $h^{ab} = g^{ab} + n^a n^b$

```
In[55]:= ΠAB = Simplify[Table[gAB[[i, j]] + na[[i]] * na[[j]], {i, 1, 4}, {j, 1, 4}]];
MatrixForm[%]
hAB = Table[ΠAB[[i + 1, j + 1]], {i, 1, 3}, {j, 1, 3}];
```

```
Out[56]/MatrixForm=
(
  0      0      0
  0      (4 M^2 r^2)/((r^2 + a^2 Cos[ø]^2) (r (2 M + r) + a^2 Cos[ø]^2)) + (2 (a^2 + r (-2 M + r)))/(a^2 + 2 r^2 + a^2 Cos[2 ø])      (2 a M r)/((a^2 + r^2) (r (2 M + r) + a^2 Cos[ø]^2))
  0      0      2/(a^2 + 2 r^2 + a^2 Cos[2 ø])
  0      (2 a M r)/((a^2 + r^2) (r (2 M + r) + a^2 Cos[ø]^2))      0      ((a^2 + r (2 M + r)) (a^2 + 2 r^2 + a^2 Cos[2 ø]) Csc[ø]^2)/(2 (a^2 + r^2)^2 (r (2 M + r) + a^2 Cos[ø]^2))
)
```

Operator projecting into the hypersurface

```
In[58]:= ΠAb = Simplify[Table[gAb[[i, j]] + na[[i]] * na[[j]], {i, 1, 4}, {j, 1, 4}]];
MatrixForm[%]
```

```
Out[59]/MatrixForm=
(
  0      0 0 0
  (2 M r)/(r (2 M + r) + a^2 Cos[ø]^2)      1 0 0
  0      0 1 0
  -(2 a M r)/((a^2 + r^2) (r (2 M + r) + a^2 Cos[ø]^2))      0 0 1
)
```

Induced metric on the hypersurface

```
In[60]:= hab = Inverse[hAB];
```

Compare asymptotic expansion with fall-off conditions in Csukás, Rácz 2020 Class. Quantum Grav. 37 155006

```
In[61]:= Series[hAB, {r, ∞, 1}] // Quiet // MatrixForm
```

```
Out[61]/MatrixForm=
(
  1 + (2 M)/r + O[1/r]^2      0      -(2 (a M Sin[ø]^2))/r + O[1/r]^2
  0      r^2 + 1/2 (a^2 + a^2 Cos[2 ø]) + O[1/r]^2      0
  -(2 (a M Sin[ø]^2))/r + O[1/r]^2      0      Sin[ø]^2 r^2 + 1/2 (a^2 Sin[ø]^2 + 2 a^2 Cos[ø]^2 Sin[ø]^2 - a^2 Cos[2 ø] Sin[ø]^2) - (2 (-a^2 M Sin[ø]^2 + a^2 M Cos[ø]^2 Sin[ø]^2))/r + O[1/r]^2
)
```

```
In[62]:= hAb = Table[Sum[hAB[[i, ii]] * hab[[ii, j]], {ii, 1, 3}], {i, 1, 3}, {j, 1, 3}] // Simplify ;
```

■ Lapse and shift

The evolution vector field is chosen to be  $t^a = (\partial_t)^a$

```
In[63]:= tA = {1, 0, 0, 0};

which satisfies  $t^a \partial_a t = 1$ 
```

In[64]:= Sum[tA[[i i]] \* D[t, xA[[i i]], {i i, 1, 4}] == 1

Out[64]= True

Lapse is given by  $N = -t^a n_a$

In[65]:= NN = -Sum[tA[[i i]] \* na[[i i]], {i i, 1, 4}]

Out[65]= 
$$\frac{1}{\sqrt{1 + \frac{2 M r}{r^2 + a^2 \cos[\vartheta]^2}}}$$

In[66]:= NNH = -Sum[tA[[i i]] \* naH[[i i]], {i i, 1, 4}]

Out[66]= 
$$\frac{1}{\sqrt{1 + 2 H[r, \vartheta]}}$$

In[67]:= CHECK == Simplify[NN Sum[nA[[i i]] \* D[t, xA[[i i]], {i i, 1, 4}]] - 1

Out[67]= CHECK == 0

Shift is given by  $N^a = \Gamma^a_b t^b$

In[68]:= NNA = Table[Sum[NAb[[i, i i]] \* tA[[i i]], {i i, 1, 4}], {i, 1, 4}]  
NNa = Simplify[Table[Sum[hAB[[i, i i]] \* NNA[[i i + 1]], {i i, 1, 3}], {i, 1, 3}]]

Out[68]= 
$$\left\{0, \frac{2 M r}{r (2 M + r) + a^2 \cos[\vartheta]^2}, 0, -\frac{2 a M r}{(a^2 + r^2) (r (2 M + r) + a^2 \cos[\vartheta]^2)}\right\}$$

Out[69]= 
$$\left\{\frac{2 M r}{a^2 + r^2}, 0, -\frac{4 a M r \sin[\vartheta]^2}{a^2 + 2 r^2 + a^2 \cos[2 \vartheta]}\right\}$$

$t^a = N n^a + N^a$

In[70]:= CHECK == MatrixForm[Table[tA[[i]] - NN nA[[i]] - NNA[[i]], {i, 1, 4}] // Simplify]

Out[70]= 
$$\text{CHECK} == \begin{pmatrix} 0 \\ 0 \\ 0 \\ 0 \end{pmatrix}$$

## ■ Extrinsic curvature

In order to compute extrinsic curvature we need the connection compatible with  $h_{ab}$ . The coordinates on the hypersurface are  $(r, \vartheta, \varphi)$

In[71]:= yA = Table[xA[[i + 1]], {i, 1, 3}]

Out[71]= {r,  $\vartheta$ ,  $\varphi$ }

In[72]:=  $\Gamma_{hab}C = \text{Table}\left[\text{Simplify}\left[\frac{1}{2} \text{Sum}[hAB[[k, i i]] * (D[hAB[[i, i i]], yA[[j j]] + D[hAB[[j, i i]], yA[[i i]] - D[hAB[[j, i]], yA[[i i]]]), \{i i, 1, 3\}], \{i, 1, 3\}, \{j, 1, 3\}, \{k, 1, 3\}\right];\right.$

In[73]:=  $\Gamma_{hAbc} = \text{Table}\left[\text{Simplify}\left[\frac{1}{2} \text{Sum}[hAB[[i, i i]] * (D[hAB[[k, i i]], yA[[j j]] + D[hAB[[j, i i]], yA[[k k]] - D[hAB[[j, k]], yA[[i i]]]), \{i i, 1, 3\}], \{i, 1, 3\}, \{j, 1, 3\}, \{k, 1, 3\}\right];\right.$

## Computing extrinsic curvature method 1

First we use the formula

$$K_{ab} = h^e_a h^f_b \nabla_e n_f = -N h^e_a h^f_b [\partial_e \partial_f t - \Gamma^c_{ef} \partial_c t] = N \Gamma^t_{ab}$$

In[74]:= Kab = NN Table[GammaAbc[[1, i, j]], {i, 2, 4}, {j, 2, 4}];  
MatrixForm[Simplify[%]]

Out[75]/MatrixForm= 
$$\left(\begin{array}{ccc} -\frac{M(a^4 + a^2 M r - 2 r^3 (M + r) + a^2 (a^2 + M r) \cos[2 \vartheta])}{(a^2 + r^2)^2 (r^2 + a^2 \cos[\vartheta]^2) \sqrt{1 + \frac{2 M r}{r^2 + a^2 \cos[\vartheta]^2}}} & -\frac{a^2 M r \sin[2 \vartheta]}{(a^2 + r^2) (r^2 + a^2 \cos[\vartheta]^2) \sqrt{1 + \frac{2 M r}{r^2 + a^2 \cos[\vartheta]^2}}} & \frac{2 a M (a^4 + a^2 (2 M - 3 r) r - 2 r^3 (2 M + 3 r) + a^2 (a^2 + (2 M - r) r) \cos[2 \vartheta]) \sin[\vartheta]^2}{(a^2 + r^2) \sqrt{1 + \frac{2 M r}{r^2 + a^2 \cos[\vartheta]^2}} (a^2 + 2 r^2 + a^2 \cos[2 \vartheta])^2} \\ -\frac{a^2 M r \sin[2 \vartheta]}{(a^2 + r^2) (r^2 + a^2 \cos[\vartheta]^2) \sqrt{1 + \frac{2 M r}{r^2 + a^2 \cos[\vartheta]^2}}} & -\frac{2 M r^2}{(r^2 + a^2 \cos[\vartheta]^2) \sqrt{1 + \frac{2 M r}{r^2 + a^2 \cos[\vartheta]^2}}} & \frac{8 a^3 M r \cos[\vartheta] \sin[\vartheta]^3}{\sqrt{1 + \frac{2 M r}{r^2 + a^2 \cos[\vartheta]^2}} (a^2 + 2 r^2 + a^2 \cos[2 \vartheta])^2} \\ \frac{2 a M (a^4 + a^2 (2 M - 3 r) r - 2 r^3 (2 M + 3 r) + a^2 (a^2 + (2 M - r) r) \cos[2 \vartheta]) \sin[\vartheta]^2}{(a^2 + r^2) \sqrt{1 + \frac{2 M r}{r^2 + a^2 \cos[\vartheta]^2}} (a^2 + 2 r^2 + a^2 \cos[2 \vartheta])^2} & \frac{8 a^3 M r \cos[\vartheta] \sin[\vartheta]^3}{\sqrt{1 + \frac{2 M r}{r^2 + a^2 \cos[\vartheta]^2}} (a^2 + 2 r^2 + a^2 \cos[2 \vartheta])^2} & -\frac{2 M r \sin[\vartheta]^2 (r^5 + a^4 r \cos[\vartheta] - a^2 M r^2 \sin[\vartheta]^2 + \cos[\vartheta]^2 (2 a^2 r^3 + a^4 M \sin[\vartheta]^2))}{(r^2 + a^2 \cos[\vartheta]^2)^3 \sqrt{1 + \frac{2 M r}{r^2 + a^2 \cos[\vartheta]^2}}} \end{array}\right)$$

In[76]:= KAB = Table[Sum[hAB[[i, i i]] \* hAB[[j, j j]] \* Kab[[i i, j j]], {i i, 1, 3}, {j j, 1, 3}], {i, 1, 3}, {j, 1, 3}] // Simplify;

## Computing extrinsic curvature method 2

Now we use

$$K_{ab} = \frac{1}{2 N} [\dot{h}_{ab} - (D_a N_b + D_b N_a)]$$

In[77]:=  $K2ab = \frac{1}{2 NN} \text{Table}[(D[hAB[[j, i]], xA[[1]]] - (D[NNa[[j]], yA[[i]] + D[NNa[[i]], yA[[j]]] - 2 \text{Sum}[\Gamma_{hab}C[[i, j, i i]] * NNa[[i i]], \{i i, 1, 3\}]]), \{i, 1, 3\}, \{j, 1, 3\}];$

```
In[78]:= CHECK == MatrixForm[Simplify[(Kab - K2ab)]]

Out[78]= CHECK == 
$$\begin{pmatrix} 0 & 0 & 0 \\ 0 & 0 & 0 \\ 0 & 0 & 0 \end{pmatrix}$$

```

## 2+1 decomposition

Now we consider  $\rho=\text{const}$  surfaces inside  $\Sigma$ .

### ■ Unit normal and induced metric

The normal 1-form is given by  $(dr)_a$

```
In[79]:= dρa = {1, 0, 0};

In[80]:= dρA = Table[Sum[hAB[[i, ii]] * dρa[[ii]], {ii, 1, 3}], {i, 1, 3}] // FullSimplify

Out[80]= 
$$\left\{ \frac{2(a^2 + r^2)}{a^2 + 2r^2 + a^2 \cos[2\vartheta]} - \frac{4Mr}{a^2 + 2r(2M+r) + a^2 \cos[2\vartheta]}, 0, \frac{2aMr}{(a^2 + r^2)(r(2M+r) + a^2 \cos[\vartheta]^2)} \right\}$$

```

The unit normal  $\hat{n}_a$  is then

```
In[81]:= nha = dρa / Sqrt[Sum[hAB[[i, j]] * dρa[[i]] * dρa[[j]], {i, 1, 3}, {j, 1, 3}]]

Out[81]= 
$$\left\{ \frac{1}{\sqrt{\frac{4M^2r^2}{(r^2+a^2\cos[\vartheta]^2)(r(2M+r)+a^2\cos[\vartheta]^2)} + \frac{2(a^2+r(-2M+r))}{a^2+2r^2+a^2\cos[2\vartheta]} }}, 0, 0 \right\}$$

```

In  $a \rightarrow 0$  limit we recover Schwarzschild

```
In[82]:= nha /. a -> 0 // Simplify

Out[82]= 
$$\left\{ \frac{1}{\sqrt{\frac{r}{2M+r}}}, 0, 0 \right\}$$

```

```
In[83]:= nhA = Table[Sum[hAB[[i, ii]] * nha[[ii]], {ii, 1, 3}], {i, 1, 3}] // Simplify

Out[83]= 
$$\left\{ \sqrt{\frac{4M^2r^2}{(r^2+a^2\cos[\vartheta]^2)(r(2M+r)+a^2\cos[\vartheta]^2)} + \frac{2(a^2+r(-2M+r))}{a^2+2r^2+a^2\cos[2\vartheta]}}, 0, \frac{2aMr}{(a^2+r^2)(r(2M+r)+a^2\cos[\vartheta]^2) \sqrt{\frac{4M^2r^2}{(r^2+a^2\cos[\vartheta]^2)(r(2M+r)+a^2\cos[\vartheta]^2)} + \frac{2(a^2+r(-2M+r))}{a^2+2r^2+a^2\cos[2\vartheta]}}} \right\}$$

```

```
In[84]:= CHECK == Sum[nha[[ii]] * nhA[[ii]], {ii, 1, 3}] - (1) // Simplify

Out[84]= CHECK == 0
```

Induced inverse metric  $\hat{\gamma}^{ab} = h^{ab} - \hat{n}^a \hat{n}^b$

```
In[85]:= πAB = Simplify[Table[hAB[[i, j]] - nhA[[i]] * nhA[[j]], {i, 1, 3}, {j, 1, 3}]];
MatrixForm[%]
MatrixForm[% /. a -> 0]
γhAB = Table[πAB[[i + 1, j + 1]], {i, 1, 2}, {j, 1, 2}];
```

```
Out[86]//MatrixForm= 
$$\begin{pmatrix} 0 & 0 & 0 \\ 0 & \frac{2}{a^2+2r^2+a^2\cos[2\vartheta]} & 0 \\ 0 & 0 & \frac{(a^2+2r^2+a^2\cos[2\vartheta])\csc[\vartheta]^2}{a^4+2r^4+a^2r(2M+3r)+a^2(a^2+r(-2M+r))\cos[2\vartheta]} \end{pmatrix}$$

```

```
Out[87]//MatrixForm= 
$$\begin{pmatrix} 0 & 0 & 0 \\ 0 & \frac{1}{r^2} & 0 \\ 0 & 0 & \frac{\csc[\vartheta]^2}{r^2} \end{pmatrix}$$

```

Operator  $\pi^a_b$  projecting into the 2-surfaces

```
In[89]:= πAb = Simplify[Table[hAb[[i, j]] - nhA[[i]] * nha[[j]], {i, 1, 3}, {j, 1, 3}]];
MatrixForm[%]

Out[90]//MatrixForm= 
$$\begin{pmatrix} 0 & 0 & 0 \\ 0 & 1 & 0 \\ -\frac{2aMr(a^2+2r^2+a^2\cos[2\vartheta])}{(a^2+r^2)(a^4+2r^4+a^2r(2M+3r)+a^2(a^2+r(-2M+r))\cos[2\vartheta])} & 0 & 1 \end{pmatrix}$$

```

Induced metric  $\hat{\gamma}_{ab}$

```
In[91]:= yhab = Inverse[yhAB] // Simplify ;
MatrixForm[%]
MatrixForm[% /. a -> 0]
```

Out[92]/MatrixForm=

$$\begin{pmatrix} \frac{1}{2} (a^2 + 2 r^2 + a^2 \cos[2 \vartheta]) & 0 \\ 0 & \frac{(a^4 + 2 r^4 + a^2 r (2 M + 3 r) + a^2 (a^2 + r (-2 M + r)) \cos[2 \vartheta]) \sin[\vartheta]^2}{a^2 + 2 r^2 + a^2 \cos[2 \vartheta]} \end{pmatrix}$$

Out[93]/MatrixForm=

$$\begin{pmatrix} r^2 & 0 \\ 0 & r^2 \sin[\vartheta]^2 \end{pmatrix}$$

## ■ Secondary lapse and shift

Evolution vector  $\rho^a = (\partial_r)^a$

```
In[94]:= rhoA = {1, 0, 0};
which satisfies rho^a partial_a r = 1
```

In[95]:= Sum[rhoA[[ii]] \* D[r, yA[[ii]]], {ii, 1, 3}] == 1

Out[95]= True

```
In[96]:= rhoa = Table[Sum[rhoA[[ii]] * hab[[ii, i]], {ii, 1, 3}], {i, 1, 3}];
Lapse N^hat
```

In[97]:= Nh = Sum[rhoA[[ii]] \* nha[[ii]], {ii, 1, 3}]

% /. a -> 0 // Simplify

Out[97]=

$$\frac{1}{\sqrt{\frac{4 M^2 r^2}{(r^2 + a^2 \cos[\vartheta]^2) (r (2 M + r) + a^2 \cos[\vartheta]^2)} + \frac{2 (a^2 + r (-2 M + r))}{a^2 + 2 r^2 + a^2 \cos[2 \vartheta]}}}$$

Out[98]=

$$\frac{1}{\sqrt{\frac{r}{2 M + r}}}$$

Shift N^hat^a

```
In[99]:= NhA = Table[Sum[piAb[[i, ii]] * rhoA[[ii]], {ii, 1, 3}], {i, 1, 3}]
Nha = Table[Sum[yhab[[i, ii]] * NhA[[ii + 1]], {ii, 1, 2}], {i, 1, 2}] // Simplify
```

Out[99]=

$$\left\{0, 0, -\frac{2 a M r (a^2 + 2 r^2 + a^2 \cos[2 \vartheta])}{(a^2 + r^2) (a^4 + 2 r^4 + a^2 r (2 M + 3 r) + a^2 (a^2 + r (-2 M + r)) \cos[2 \vartheta])}\right\}$$

Out[100]=

$$\left\{0, -\frac{2 a M r \sin[\vartheta]^2}{a^2 + r^2}\right\}$$

```
In[101]:= CHECK == Nh Sum[nhA[[ii]] * D[r, yA[[ii]]], {ii, 1, 3}] - 1
```

Out[101]= CHECK == 0

$\rho^a = \hat{N} \hat{n}^a + \hat{N}^a$

```
In[102]:= CHECK == MatrixForm[Table[rhoA[[i]] - Nh nha[[i]] - NhA[[i]], {i, 1, 3}] // Simplify]
```

Out[102]=

$$\begin{pmatrix} 0 \\ 0 \\ 0 \end{pmatrix}$$

```
In[103]:= CHECK == MatrixForm[Simplify[hAB - (piAB + Table[Nh^-2 (rhoA[[i]] - NhA[[i]]) * (rhoA[[j]] - NhA[[j]]), {i, 1, 3}, {j, 1, 3}])]]
```

Out[103]=

$$\begin{pmatrix} 0 & 0 & 0 \\ 0 & 0 & 0 \\ 0 & 0 & 0 \end{pmatrix}$$

```
In[104]:= CHECK == MatrixForm[Simplify[
hab - ({Nh^2 + Sum[yhAB[[i, j]] * Nha[[i]] * Nha[[j]], {i, 1, 2}, {j, 1, 2}], Nha[[1]], Nha[[2]], Join[{Nha[[1]], yhab[[1]], Join[{Nha[[2]], yhab[[2]]}]]]

```

Out[104]=

$$\begin{pmatrix} 0 & 0 & 0 \\ 0 & 0 & 0 \\ 0 & 0 & 0 \end{pmatrix}$$

## ■ Secondary extrinsic curvature

In order to compute exterior curvature we need the connection compatible with  $\hat{\gamma}_{ab}$ . The coordinates on S are  $(\vartheta, \varphi)$

```
In[105]:= zA = Table[yA[[i + 1]], {i, 1, 2}]
```

Out[105]= {ϑ, ϕ}

```
In[106]:= ΓyhabC = Table[Simplify[ $\frac{1}{2}$  Sum[γhAB[[k, ii]] × (D[γhab[[i, ii]], zA[[j]] + D[γhab[[j, ii]], zA[[i]] - D[γhab[[j, i]], zA[[ii]]), {ii, 1, 2}]],  
{i, 1, 2}, {j, 1, 2}, {k, 1, 2}];  
ΓyhAbc = Table[Simplify[ $\frac{1}{2}$  Sum[γhAB[[i, ii]] × (D[γhab[[k, ii]], zA[[j]] + D[γhab[[j, ii]], zA[[k]] - D[γhab[[j, k]], zA[[ii]]), {ii, 1, 2}]],  
{i, 1, 2}, {j, 1, 2}, {k, 1, 2}];
```

## Computing extrinsic curvature method 1

First we use the formula

$$\hat{K}_{ab} = \hat{\gamma}^e{}_a \hat{\gamma}^f{}_b D_e \hat{n}_f = \hat{N} \hat{\gamma}^e{}_a \hat{\gamma}^f{}_b [\partial_e \partial_f \rho - \Gamma h^c{}_{ef} \partial_c \rho] = -\hat{N} \Gamma h^\rho{}_{ab}$$

```
In[108]:= Khab = -Nh Table[ΓhAbc[[1, i, j]], {i, 2, 3}, {j, 2, 3}];  
MatrixForm[Simplify[%]];  
MatrixForm[%] // Simplify  
MatrixForm[% /. a -> 0] // Simplify
```

Out[110]//MatrixForm=

$$\left( \begin{array}{cc} \frac{\frac{4 M^2 r^3}{(r^2 + a^2 \cos[\theta]^2) (r (2 M + r) + a^2 \cos[\theta]^2)} + \frac{2 r (a^2 + r (-2 M + r))}{a^2 + 2 r^2 + a^2 \cos[2 \theta]}}{\sqrt{\frac{4 M^2 r^2}{(r^2 + a^2 \cos[\theta]^2) (r (2 M + r) + a^2 \cos[\theta]^2)} + \frac{2 (a^2 + r (-2 M + r))}{a^2 + 2 r^2 + a^2 \cos[2 \theta]}}} & - \frac{32 a^3 M^2 r^2 \cos[\theta] \sin[\theta]^3}{(a^2 + 2 r^2 + a^2 \cos[2 \theta])^2 (a^2 + 2 r (2 M + r) + a^2 \cos[2 \theta]) \sqrt{\frac{4 M^2 r^2}{(r^2 + a^2 \cos[\theta]^2) (r (2 M + r) + a^2 \cos[\theta]^2)} + \frac{2 (a^2 + r (-2 M + r))}{a^2 + 2 r^2 + a^2 \cos[2 \theta]}}} \\ - \frac{32 a^3 M^2 r^2 \cos[\theta] \sin[\theta]^3}{(a^2 + 2 r^2 + a^2 \cos[2 \theta])^2 (a^2 + 2 r (2 M + r) + a^2 \cos[2 \theta]) \sqrt{\frac{4 M^2 r^2}{(r^2 + a^2 \cos[\theta]^2) (r (2 M + r) + a^2 \cos[\theta]^2)} + \frac{2 (a^2 + r (-2 M + r))}{a^2 + 2 r^2 + a^2 \cos[2 \theta]}}} & - \frac{32 a^3 M^2 r^2 \cos[\theta] \sin[\theta]^3}{(a^2 + 2 r^2 + a^2 \cos[2 \theta])^2 (a^2 + 2 r (2 M + r) + a^2 \cos[2 \theta]) \sqrt{\frac{4 M^2 r^2}{(r^2 + a^2 \cos[\theta]^2) (r (2 M + r) + a^2 \cos[\theta]^2)} + \frac{2 (a^2 + r (-2 M + r))}{a^2 + 2 r^2 + a^2 \cos[2 \theta]}}} \end{array} \right)$$

Out[111]//MatrixForm=

$$\left( \begin{array}{cc} r \sqrt{\frac{r}{2 M + r}} & 0 \\ 0 & r \sqrt{\frac{r}{2 M + r}} \sin[\theta]^2 \end{array} \right)$$

Its trace  $\hat{K}$  is

```
In[112]:= Khat = Sum[γhAB[[ii, jj]] × Khab[[ii, jj]], {ii, 1, 2}, {jj, 1, 2}] // Simplify  
% /. a -> 0
```

Out[112]=

$$\frac{\sqrt{2} (4 r^3 + a^2 (M + 3 r) - a^2 (M - r) \cos[2 \theta])}{(a^2 + 2 r^2 + a^2 \cos[2 \theta]) (a^2 + 2 r (2 M + r) + a^2 \cos[2 \theta]) \sqrt{\frac{a^4 + 2 r^4 + a^2 r (2 M + 3 r) + a^2 (a^2 + r (-2 M + r)) \cos[2 \theta]}{(a^2 + 2 r^2 + a^2 \cos[2 \theta]) (a^2 + 2 r (2 M + r) + a^2 \cos[2 \theta])}}}$$

Out[113]=

$$\frac{2}{\sqrt{\frac{r}{2 M + r}} (2 M + r)}$$

```
In[114]:= KhAB = Table[Sum[Khab[[ii, jj]] × γhAB[[ii, i]] × γhAB[[jj, j]], {ii, 1, 2}, {jj, 1, 2}], {i, 1, 2}, {j, 1, 2}] // Simplify ;  
MatrixForm[%]
```

Out[115]//MatrixForm=

$$\left( \begin{array}{cc} - \frac{4 \left( - \frac{4 M^2 r^3}{(r^2 + a^2 \cos[\theta]^2) (r (2 M + r) + a^2 \cos[\theta]^2)} - \frac{2 r (a^2 + r (-2 M + r))}{a^2 + 2 r^2 + a^2 \cos[2 \theta]} \right)}{(a^2 + 2 r^2 + a^2 \cos[2 \theta])^2 \sqrt{\frac{4 M^2 r^2}{(r^2 + a^2 \cos[\theta]^2) (r (2 M + r) + a^2 \cos[\theta]^2)} + \frac{2 (a^2 + r (-2 M + r))}{a^2 + 2 r^2 + a^2 \cos[2 \theta]}}} & - \frac{32 \sqrt{2} a^3 M^2 r^2 \cos[\theta] \sqrt{\frac{a^4 + 2 r^4 + a^2 r (2 M + 3 r) + a^2 (a^2 + r (-2 M + r)) \cos[2 \theta]}{(a^2 + 2 r^2 + a^2 \cos[2 \theta]) (a^2 + 2 r (2 M + r) + a^2 \cos[2 \theta])}} \sin[\theta]}{(a^2 + 2 r^2 + a^2 \cos[2 \theta]) (a^4 + 2 r^4 + a^2 r (2 M + 3 r) + a^2 (a^2 + r (-2 M + r)) \cos[2 \theta])^2} \\ - \frac{32 \sqrt{2} a^3 M^2 r^2 \cos[\theta] \sqrt{\frac{a^4 + 2 r^4 + a^2 r (2 M + 3 r) + a^2 (a^2 + r (-2 M + r)) \cos[2 \theta]}{(a^2 + 2 r^2 + a^2 \cos[2 \theta]) (a^2 + 2 r (2 M + r) + a^2 \cos[2 \theta])}} \sin[\theta]}{(a^2 + 2 r^2 + a^2 \cos[2 \theta]) (a^4 + 2 r^4 + a^2 r (2 M + 3 r) + a^2 (a^2 + r (-2 M + r)) \cos[2 \theta])^2} & - \frac{\sqrt{\frac{a^4 + 2 r^4 + a^2 r (2 M + 3 r) + a^2 (a^2 + r (-2 M + r)) \cos[2 \theta]}{(a^2 + 2 r^2 + a^2 \cos[2 \theta]) (a^2 + 2 r (2 M + r) + a^2 \cos[2 \theta])}} (a^4 M + 3 a^4 r - 4 a^2 M r^2 + 8 a^2 r^3 + 8 r^5 + 4 a^2 r (a^2 + r (M + 2 r)) \cos[2 \theta] - a^4 (M - r) \cos[4 \theta]) \csc[\theta]^2}{\sqrt{2} (a^4 + 2 r^4 + a^2 r (2 M + 3 r) + a^2 (a^2 + r (-2 M + r)) \cos[2 \theta])^2} \end{array} \right)$$

## Computing extrinsic curvature method 2

Now we use

$$K_{ab} = \frac{1}{2 N} [\dot{h}_{ab} - (D_a N_b + D_b N_a)]$$

```
In[116]:= Kh2ab =  
1 / (2 Nh) Table[(D[γhab[[j, i]], yA[[1]] - (D[Nha[[j]], zA[[i]] + D[Nha[[i]], zA[[j]] - 2 Sum[ΓyhabC[[i, j, ii]] × Nha[[ii]], {ii, 1, 2}))), {i, 1, 2}, {j, 1, 2}];
```

```
In[117]:= CHECK == MatrixForm[Simplify[(Khab - Kh2ab)]]
```

Out[117]=

$$\text{CHECK} == \begin{pmatrix} 0 & 0 \\ 0 & 0 \end{pmatrix}$$

## Computing extrinsic curvature method 3

This time using  $\hat{K}_{ab} = \frac{1}{2} \mathcal{L}_{\hat{n}} \hat{\gamma}_{ab}$



```
In[118]:= Kh3ab = Table[1/2 Sum[
  (D[(hab[[i, j]] - nha[[i]]*nha[[j]]), yA[[ii]]*
  nha[[ii]]
  + (hab[[ii, j]] - nha[[ii]*nha[[j]])*D[nhA[[ii]], yA[[i]]]
  + (hab[[i, ii]] - nha[[i]*nha[[ii]])*D[nhA[[ii]], yA[[j]]]),
  {ii, 1, 3}], {i, 2, 3}, {j, 2, 3}];
```

```
In[119]:= CHECK == MatrixForm[Simplify[(Khab - Kh3ab)]]
```

```
Out[119]= CHECK ==  $\begin{pmatrix} 0 & 0 \\ 0 & 0 \end{pmatrix}$ 
```

## ■ Decomposing extrinsic curvature

Scalar projection of  $K_{ab}$

$$\kappa = \hat{n}^a \hat{n}^b K_{ab}$$

```
In[120]:=  $\kappa$  = Sum[nhA[[ii]]*nhA[[jj]]*Kab[[ii, jj], {ii, 1, 3}, {jj, 1, 3}] // Simplify
% /. a -> 0 // Simplify
```

```
Out[120]= 
$$\left( M \left( -10 a^8 - 14 a^6 M r - 24 a^6 r^2 - 28 a^4 M r^3 - 4 a^4 r^4 - 64 a^2 M^2 r^4 - 16 a^2 M r^5 + 32 a^2 r^6 + 32 M r^7 + 32 r^8 - a^2 (15 a^6 + 16 a^2 M r^3 + a^4 r (17 M + 32 r) - 16 r^4 (4 M^2 + 3 M r + 2 r^2)) \cos[2 \vartheta] - 2 a^4 (3 a^4 - 2 r^3 (3 M + r) + a^2 r (M + 4 r)) \cos[4 \vartheta] - a^8 \cos[6 \vartheta] + a^6 M r \cos[6 \vartheta] \right) \right. \\ \left. \left( \sqrt{1 + \frac{2 M r}{r^2 + a^2 \cos[\vartheta]^2}} (a^2 + 2 r^2 + a^2 \cos[2 \vartheta])^2 (a^2 + 2 r (2 M + r) + a^2 \cos[2 \vartheta]) (a^4 + 2 r^4 + a^2 r (2 M + 3 r) + a^2 (a^2 + r (-2 M + r)) \cos[2 \vartheta]) \right) \right. \\ \left. \frac{2 M (M + r)}{\sqrt{1 + \frac{2 M}{r}} r^2 (2 M + r)} \right)$$

```

Vector projection of  $K_{ab}$

$$k_a = \hat{n}^b \hat{Y}_a^c K_{bc}$$

```
In[122]:= kk3a = Table[Sum[nhA[[ii]]*piAb[[jj, i]]*Kab[[ii, jj], {ii, 1, 3}, {jj, 1, 3}], {i, 1, 3}] // Simplify ;
MatrixForm[%]
MatrixForm[% /. a -> 0]
```

```
Out[123]//MatrixForm= 
$$\begin{pmatrix} -\frac{2 a^2 M^2 r (a^4 - 3 a^2 r^2 - 6 r^4 + a^2 (a^2 - r^2) \cos[2 \vartheta]) \sin[\vartheta]^2}{(a^2 + r^2) \sqrt{\frac{1}{8} + \frac{M r}{4 (r^2 + a^2 \cos[\vartheta]^2)}} (a^2 + 2 r^2 + a^2 \cos[2 \vartheta])^3 (a^2 + 2 r (2 M + r) + a^2 \cos[2 \vartheta]) \left( \frac{a^4 + 2 r^4 + a^2 r (2 M + 3 r) + a^2 (a^2 + r (-2 M + r)) \cos[2 \vartheta]}{(a^2 + 2 r^2 + a^2 \cos[2 \vartheta]) (a^2 + 2 r (2 M + r) + a^2 \cos[2 \vartheta])} \right)^{3/2}} \\ -\frac{2 a^2 M r \sin[2 \vartheta]}{\sqrt{\frac{1}{2} + \frac{M r}{r^2 + a^2 \cos[\vartheta]^2}} (a^2 + 2 r^2 + a^2 \cos[2 \vartheta]) (a^2 + 2 r (2 M + r) + a^2 \cos[2 \vartheta]) \sqrt{\frac{a^4 + 2 r^4 + a^2 r (2 M + 3 r) + a^2 (a^2 + r (-2 M + r)) \cos[2 \vartheta]}{(a^2 + 2 r^2 + a^2 \cos[2 \vartheta]) (a^2 + 2 r (2 M + r) + a^2 \cos[2 \vartheta])}}} \\ \frac{a M (a^4 - 3 a^2 r^2 - 6 r^4 + a^2 (a^2 - r^2) \cos[2 \vartheta]) \sin[\vartheta]^2}{\sqrt{\frac{1}{8} + \frac{M r}{4 (r^2 + a^2 \cos[\vartheta]^2)}} (a^2 + 2 r^2 + a^2 \cos[2 \vartheta])^3 \sqrt{\frac{a^4 + 2 r^4 + a^2 r (2 M + 3 r) + a^2 (a^2 + r (-2 M + r)) \cos[2 \vartheta]}{(a^2 + 2 r^2 + a^2 \cos[2 \vartheta]) (a^2 + 2 r (2 M + r) + a^2 \cos[2 \vartheta])}}} \end{pmatrix}$$

```

Out[124]//MatrixForm=

$$\begin{pmatrix} 0 \\ 0 \\ 0 \end{pmatrix}$$

```
In[125]:= CHECK == Sum[kk3a[[ii]]*nhA[[ii], {ii, 1, 3}] // Simplify
```

```
Out[125]= CHECK == 0
```

```
In[126]:= kk3A = Table[Sum[hAB[[i, ii]]*kk3a[[ii], {ii, 1, 3}], {i, 1, 3}] // Simplify ;
MatrixForm[%]
```

```
Out[127]//MatrixForm= 
$$\begin{pmatrix} 0 \\ -\frac{4 a^2 M r \sin[2 \vartheta]}{\sqrt{\frac{1}{2} + \frac{M r}{r^2 + a^2 \cos[\vartheta]^2}} (a^2 + 2 r^2 + a^2 \cos[2 \vartheta])^2 (a^2 + 2 r (2 M + r) + a^2 \cos[2 \vartheta]) \sqrt{\frac{a^4 + 2 r^4 + a^2 r (2 M + 3 r) + a^2 (a^2 + r (-2 M + r)) \cos[2 \vartheta]}{(a^2 + 2 r^2 + a^2 \cos[2 \vartheta]) (a^2 + 2 r (2 M + r) + a^2 \cos[2 \vartheta])}}} \\ \frac{a M (a^4 - 3 a^2 r^2 - 6 r^4 + a^2 (a^2 - r^2) \cos[2 \vartheta])}{(r (2 M + r) + a^2 \cos[\vartheta]^2) \sqrt{\frac{2 M r + r^2 + a^2 \cos[\vartheta]^2}{2 r^2 + 2 a^2 \cos[\vartheta]^2}} (a^2 + 2 r^2 + a^2 \cos[2 \vartheta])^3 \left( \frac{a^4 + 2 r^4 + a^2 r (2 M + 3 r) + a^2 (a^2 + r (-2 M + r)) \cos[2 \vartheta]}{(a^2 + 2 r^2 + a^2 \cos[2 \vartheta]) (a^2 + 2 r (2 M + r) + a^2 \cos[2 \vartheta])} \right)^{3/2}} \end{pmatrix}$$

```

Pull back into 2-surfaces

```
In[128]:= kka = Table[Sum[nhA[[ii]] * πAb[[jj, i]] * Kab[[ii, jj]], {ii, 1, 3}, {jj, 1, 3}], {i, 2, 3}] // Simplify ;  
MatrixForm[%]  
MatrixForm[% /. a -> 0]
```

Out[129]//MatrixForm=

$$\left( \begin{array}{c} -\frac{2 a^2 M r \sin[2 \theta]}{\sqrt{\frac{1}{2}+\frac{M r}{r^2+a^2 \cos [\theta]^2}}\left(a^2+2 r^2+a^2 \cos [2 \theta]\right)\left(a^2+2 r(2 M+r)+a^2 \cos [2 \theta]\right) \sqrt{\frac{a^4+2 r^4+a^2 r(2 M+3 r)+a^2\left(a^2+r(-2 M+r)\right) \cos [2 \theta]}{\left(a^2+2 r^2+a^2 \cos [2 \theta]\right)\left(a^2+2 r(2 M+r)+a^2 \cos [2 \theta]\right)}}} \\ \frac{a M\left(a^4-3 a^2 r^2-6 r^4+a^2\left(a^2-r^2\right) \cos [2 \theta]\right) \sin [\theta]^2}{\sqrt{\frac{1}{8}+\frac{M r}{4\left(r^2+a^2 \cos [\theta]^2\right)}}\left(a^2+2 r^2+a^2 \cos [2 \theta]\right)^3 \sqrt{\frac{a^4+2 r^4+a^2 r(2 M+3 r)+a^2\left(a^2+r(-2 M+r)\right) \cos [2 \theta]}{\left(a^2+2 r^2+a^2 \cos [2 \theta]\right)\left(a^2+2 r(2 M+r)+a^2 \cos [2 \theta]\right)}}} \end{array} \right)$$

Out[130]//MatrixForm=

$$\left(\begin{array}{c} 0 \\ 0 \end{array}\right)$$

```
In[131]:= kka = Table[Sum[γhAB[[i, ii]] * kka[[ii]], {ii, 1, 2}], {i, 1, 2}] // Simplify ;  
MatrixForm[%]
```

Out[132]//MatrixForm=

$$\left( \begin{array}{c} -\frac{4 a^2 M r \sin[2 \theta]}{\sqrt{\frac{1}{2}+\frac{M r}{r^2+a^2 \cos [\theta]^2}}\left(a^2+2 r^2+a^2 \cos [2 \theta]\right)^2\left(a^2+2 r(2 M+r)+a^2 \cos [2 \theta]\right) \sqrt{\frac{a^4+2 r^4+a^2 r(2 M+3 r)+a^2\left(a^2+r(-2 M+r)\right) \cos [2 \theta]}{\left(a^2+2 r^2+a^2 \cos [2 \theta]\right)\left(a^2+2 r(2 M+r)+a^2 \cos [2 \theta]\right)}}} \\ \frac{2 a M\left(a^4-3 a^2 r^2-6 r^4+a^2\left(a^2-r^2\right) \cos [2 \theta]\right)}{\sqrt{\frac{2 M r+r^2+a^2 \cos [\theta]^2}{2 r^2+2 a^2 \cos [\theta]^2}}\left(a^2+2 r^2+a^2 \cos [2 \theta]\right)^3\left(a^2+2 r(2 M+r)+a^2 \cos [2 \theta]\right)\left(\frac{a^4+2 r^4+a^2 r(2 M+3 r)+a^2\left(a^2+r(-2 M+r)\right) \cos [2 \theta]}{\left(a^2+2 r^2+a^2 \cos [2 \theta]\right)\left(a^2+2 r(2 M+r)+a^2 \cos [2 \theta]\right)}\right)^{3 / 2}} \end{array} \right)$$

Tensor projection of  $K_{ab}$

$$\mathbb{K}_{ab} = \hat{Y}_a^e \hat{Y}_b^f K_{ef}$$

```
In[133]:= KKab = Table[Sum[πAb[[ii, i]] * πAb[[jj, j]] * Kab[[ii, jj]], {ii, 1, 3}, {jj, 1, 3}], {i, 2, 3}, {j, 2, 3}] // Simplify ;  
MatrixForm[%]  
MatrixForm[% /. a -> 0]
```

Out[134]//MatrixForm=

$$\left( \begin{array}{c} -\frac{2 M r^2}{\left(r^2+a^2 \cos [\theta]^2\right) \sqrt{1+\frac{2 M r}{r^2+a^2 \cos [\theta]^2}}} \frac{8 a^3 M r \cos [\theta] \sin [\theta]^3}{\sqrt{1+\frac{2 M r}{r^2+a^2 \cos [\theta]^2}}\left(a^2+2 r^2+a^2 \cos [2 \theta]\right)^2} \\ \frac{8 a^3 M r \cos [\theta] \sin [\theta]^3}{\sqrt{1+\frac{2 M r}{r^2+a^2 \cos [\theta]^2}}\left(a^2+2 r^2+a^2 \cos [2 \theta]\right)^2} -\frac{2 M r \sin [\theta]^2\left(r^6+a^4 r \cos [\theta]^4-a^2 M r^2 \sin [\theta]^2+\cos [\theta]^2\left(2 a^2 r^3+a^4 M \sin [\theta]^2\right)\right)}{\left(r^2+a^2 \cos [\theta]^2\right)^3 \sqrt{1+\frac{2 M r}{r^2+a^2 \cos [\theta]^2}}} \end{array} \right)$$

Out[135]//MatrixForm=

$$\left(\begin{array}{cc} -\frac{2 M}{\sqrt{1+\frac{2 M}{r}}} & 0 \\ 0 & -\frac{2 M \sin [\theta]^2}{\sqrt{1+\frac{2 M}{r}}} \end{array}\right)$$

```
In[136]:= KKAB = Table[Sum[γhAB[[i, ii]] * γhAB[[j, jj]] * KKab[[ii, jj]], {ii, 1, 2}, {jj, 1, 2}], {i, 1, 2}, {j, 1, 2}] // Simplify ;  
MatrixForm[%]  
MatrixForm[% /. a -> 0]
```

Out[137]//MatrixForm=

$$\left( \begin{array}{c} -\frac{16 M r^2}{\sqrt{1+\frac{2 M r}{r^2+a^2 \cos [\theta]^2}}\left(a^2+2 r^2+a^2 \cos [2 \theta]\right)^3} \frac{8 a^3 M r \sin[2 \theta]}{\sqrt{1+\frac{2 M r}{r^2+a^2 \cos [\theta]^2}}\left(a^2+2 r^2+a^2 \cos [2 \theta]\right)^2\left(a^4+2 r^4+a^2 r(2 M+3 r)+a^2\left(a^2+r(-2 M+r)\right) \cos [2 \theta]\right)} \\ \frac{8 a^3 M r \sin[2 \theta]}{\sqrt{1+\frac{2 M r}{r^2+a^2 \cos [\theta]^2}}\left(a^2+2 r^2+a^2 \cos [2 \theta]\right)^2\left(a^4+2 r^4+a^2 r(2 M+3 r)+a^2\left(a^2+r(-2 M+r)\right) \cos [2 \theta]\right)} -\frac{2 M r\left(a^2+2 r^2+a^2 \cos [2 \theta]\right)^2\left(a^4 \cos [\theta]^2(M+r \cot [\theta]^2)+r^2\left(-a^2 M+2 a^2 r \cot [\theta]^2+r^3 \csc [\theta]^2\right)\right)}{\left(r^2+a^2 \cos [\theta]^2\right)^3 \sqrt{1+\frac{2 M r}{r^2+a^2 \cos [\theta]^2}}\left(a^4+2 r^4+a^2 r(2 M+3 r)+a^2\left(a^2+r(-2 M+r)\right) \cos [2 \theta]\right)^2} \end{array} \right)$$

Out[138]//MatrixForm=

$$\left(\begin{array}{cc} -\frac{2 M}{\sqrt{1+\frac{2 M}{r}}} r^4 & 0 \\ 0 & -\frac{2 M \csc [\theta]^2}{\sqrt{1+\frac{2 M}{r}}} r^4 \end{array}\right)$$

Trace of tensor projection

$$\mathbb{K} = \hat{Y}^{ab} \mathbb{K}_{ab}$$

```
In[139]:= KK = Sum[γhAB[[ii, jj]] * KKab[[ii, jj]], {ii, 1, 2}, {jj, 1, 2}] // Simplify  
% /. a -> 0
```

Out[139]=

$$-\frac{4 M r\left(4 r^3+a^2(M+3 r)-a^2(M-r) \cos [2 \theta]\right)}{\sqrt{1+\frac{2 M r}{r^2+a^2 \cos [\theta]^2}}\left(a^2+2 r^2+a^2 \cos [2 \theta]\right)\left(a^4+2 r^4+a^2 r(2 M+3 r)+a^2\left(a^2+r(-2 M+r)\right) \cos [2 \theta]\right)}$$

Out[140]=

$$-\frac{4 M}{\sqrt{1+\frac{2 M}{r}}} r^2$$

Trace free part of tensorial projection

$$\overset{\circ}{\mathbb{K}}_{ab} = \mathbb{K}_{ab} - \frac{1}{2} \hat{Y}_{ab} \mathbb{K}^f{}_f$$

```
In[141]:= KKcab = Table[KKab[[i, j]] -  $\frac{1}{2} \gamma_{hab}[[i, j]] \text{KK}[\{i, 1, 2\}, \{j, 1, 2\}] // \text{Simplify};$ 
```

```
MatrixForm[%]
```

```
Out[142]//MatrixForm=
```

$$\begin{pmatrix} \frac{a^2 M r (a^2 (M-r) - 2 r^2 (3 M+r) + a^2 (M-r) \cos[2 \vartheta]) \sin[\vartheta]^2}{(r^2 + a^2 \cos[\vartheta]^2) \sqrt{1 + \frac{2 M r}{r^2 + a^2 \cos[\vartheta]^2} (a^4 + 2 r^4 + a^2 r (2 M + 3 r) + a^2 (a^2 + r (-2 M + r)) \cos[2 \vartheta])}} & \frac{8 a^3 M r \cos[\vartheta] \sin[\vartheta]^3}{\sqrt{1 + \frac{2 M r}{r^2 + a^2 \cos[\vartheta]^2} (a^2 + 2 r^2 + a^2 \cos[2 \vartheta])^2}} \\ \frac{8 a^3 M r \cos[\vartheta] \sin[\vartheta]^3}{\sqrt{1 + \frac{2 M r}{r^2 + a^2 \cos[\vartheta]^2} (a^2 + 2 r^2 + a^2 \cos[2 \vartheta])^2}} & \frac{4 a^2 M r (a^2 (-M+r) + 2 r^2 (3 M+r) - a^2 (M-r) \cos[2 \vartheta]) \sin[\vartheta]^4}{\sqrt{1 + \frac{2 M r}{r^2 + a^2 \cos[\vartheta]^2} (a^2 + 2 r^2 + a^2 \cos[2 \vartheta])^3}} \end{pmatrix}$$

```
In[143]:= KKcAB = Table[Sum[KKcab[[ii, jj]] *  $\gamma_{hAB}[[ii, i]]$  *  $\gamma_{hAB}[[jj, j]]$ , {ii, 1, 2}, {jj, 1, 2}], {i, 1, 2}, {j, 1, 2}] // Simplify;
```

```
In[144]:= CHECK == MatrixForm[Simplify[KAB - (Table[nhA[[i]] * nhA[[j]]  $\kappa\kappa$ , {i, 1, 3}, {j, 1, 3}] + Table[nhA[[i]] * Join[{0}, kkA][[j]], {i, 1, 3}, {j, 1, 3}] +
```

```
Table[nhA[[j]] * Join[{0}, kkA][[i]], {i, 1, 3}, {j, 1, 3}] + {{0, 0, 0}, Join[{0}, KKcAB[[1]], Join[{0}, KKcAB[[2]]] +  $\frac{1}{2} \text{KK} \pi_{AB}$  }]]]
```

```
Out[144]= CHECK ==  $\begin{pmatrix} 0 & 0 & 0 \\ 0 & 0 & 0 \\ 0 & 0 & 0 \end{pmatrix}$ 
```

Series expansion of  $\frac{K}{K}$  is in accordance with the hyperbolicity condition of Beyer et al.

```
In[145]:= Series[Simplify[ $\frac{KK}{KK}$ ], {r,  $\infty$ , 3}]
```

```
Out[145]=  $-\frac{1}{2} + \frac{M}{2 r} + \frac{3 a^2 - 8 M^2 + a^2 \cos[2 \vartheta]}{8 r^2} + \frac{2 M^3 - a^2 M \cos[2 \vartheta]}{r^3} + O\left[\frac{1}{r}\right]^4$ 
```

## Spin-weighted variables

We have to supply the code with  $a, b, \mathbb{R}(=2), \hat{\mathbb{N}}, \mathbb{N}, k, K, K_{qq}^{\circ}$  and  $\kappa$ . Once having these, it can compute all the other variables.

### ■ Dyad

On the unit sphere we have the complex dyad  $\{q^a, \bar{q}^a\}$

```
In[146]:= qA = -{1,  $\frac{J}{\sin[\vartheta]}$ };
```

```
qbA = -{1,  $-\frac{J}{\sin[\vartheta]}$ };
```

```
qa = -{1, J Sin[ $\vartheta$ ]};
```

```
qba = -{1, -J Sin[ $\vartheta$ ]};
```

Then the normalization  $q^a q_a = 0 = \bar{q}^a \bar{q}_a$  and  $q^a \bar{q}_a = 2$

```
In[150]:= Sum[qA[[ii]] * qa[[ii]], {ii, 1, 2}] /. J^2 -> -1
Sum[qbA[[ii]] * qba[[ii]], {ii, 1, 2}] /. J^2 -> -1
Sum[qA[[ii]] * qba[[ii]], {ii, 1, 2}] /. J^2 -> -1
```

```
Out[150]= 0
```

```
Out[151]= 0
```

```
Out[152]= 2
```

Unit sphere metric can be written as  $q_{ab} = q_{(a} \bar{q}_{b)}$

```
In[153]:= qab = Table[ $\frac{1}{2} (qa[[i]] * qba[[j]] + qa[[j]] * qba[[i]])$ , {i, 1, 2}, {j, 1, 2}] /. J^2 -> -1;
```

```
MatrixForm[%]
```

```
Out[154]//MatrixForm=
```

$$\begin{pmatrix} 1 & 0 \\ 0 & \sin[\vartheta]^2 \end{pmatrix}$$

```
In[155]:= qAB = Inverse[qab];
```

```
qAb = Table[KroneckerDelta[i, j], {i, 1, 2}, {j, 1, 2}];
```

We define them on the whole initial data surface by Lie dragging them along  $\rho^a$

```
In[157]:= qpA = -{0, 1,  $\frac{J}{\sin[\vartheta]}$ };
```

```
qpbA = -{0, 1,  $-\frac{J}{\sin[\vartheta]}$ };
```

```
qpA = -{0, 1, J Sin[ $\vartheta$ ]};
```

```
qpbA = -{0, 1, -J Sin[ $\vartheta$ ]};
```

$\mathcal{L}_\rho q^a = 0$

```
In[161]:= Table[Sum[ρA[[ii]] × (D[qpA[[i]], yA[[ii]]) + Sum[ΓhAbc[[i, jj, ii]] × qpA[[jj]], {jj, 1, 3}]), {ii, 1, 3}] -
      Sum[qpA[[ii]] × (D[ρA[[i]], yA[[ii]]) + Sum[ΓhAbc[[i, jj, ii]] × ρA[[jj]], {jj, 1, 3}]), {ii, 1, 3}], {i, 1, 3}] // Simplify
Out[161]= {0, 0, 0}


$$\mathcal{L}_\rho q_a = 0$$


In[162]:= Table[Sum[ρA[[ii]] × (D[qpA[[i]], yA[[ii]]) - Sum[ΓhAbc[[jj, i, ii]] × qpa[[jj]], {jj, 1, 3}]), {ii, 1, 3}] +
      Sum[qpa[[ii]] × (D[ρA[[ii]], yA[[i]]) + Sum[ΓhAbc[[ii, jj, i]] × ρA[[jj]], {jj, 1, 3}]), {ii, 1, 3}], {i, 1, 3}] // Simplify
Out[162]= {0, 0, 0}

Connection compatible with the unit sphere metric and its curvature

In[163]:= ΓqAbc = Table[
      Simplify[ $\frac{1}{2}$  Sum[qAB[[i, ii]] × (D[qab[[k, ii]], zA[[j]] + D[qab[[j, ii]], zA[[k]] - D[qab[[j, k]], zA[[ii]]]), {ii, 1, 2}]], {i, 1, 2}, {j, 1, 2}, {k, 1, 2}];

In[164]:= RqabcD = Table[-D[ΓqAbc[[l, j, k]], zA[[i]] + D[ΓqAbc[[l, i, k]], zA[[j]] +
      Sum[-ΓqAbc[[l, i, ii]] × ΓqAbc[[ii, j, k]] + ΓqAbc[[l, j, ii]] × ΓqAbc[[ii, i, k]], {ii, 1, 2}], {i, 1, 2}, {j, 1, 2}, {k, 1, 2}, {l, 1, 2}];

In[165]:= Rqab = Table[Sum[RqabcD[[i, ii, j, ii]], {ii, 1, 2}], {i, 1, 2}, {j, 1, 2}] // Simplify
Out[165]= {{1, 0}, {0, Sin[ϑ]^2}}

In[166]:= Simplify[Sum[Rqab[[ii, jj]] × qAB[[ii, jj]], {ii, 1, 2}, {jj, 1, 2}]]
Out[166]= 2
```

## ■ Induced metric

$h_{ab}$  is decomposed into  $\hat{N}, \hat{N}^a$  and  $\hat{\gamma}_{ab}$ .  $\hat{N}$  is a spin-weight 0 function but  $\hat{N}_a$  is projected into spin-weight 1  $\mathbb{N} = q^a \hat{N}_a$  and  $\hat{\gamma}_{ab}$  is projected into spin-weight 0  $\mathbf{a} = \frac{1}{2} \hat{\gamma}_{ab} q^a \bar{q}^b$  and spin-weight 2  $\mathbf{b} = \frac{1}{2} \hat{\gamma}_{ab} q^a q^b$ .

Asymptotic behaviour of  $\hat{N}$  is compatible with the derived fall-off conditions

```
In[168]:= Series[Nh, {r, ∞, 1}]
Out[168]= 1 +  $\frac{M}{r}$  + O[ $\frac{1}{r}$ ]2


$$\mathbb{N} = q^a \hat{N}_a$$


In[172]:= N = Sum[Nha[[ii]] × qA[[ii]], {ii, 1, 2}] // Simplify
Nbar = N /. J → -J;


$$\frac{2 a J M r \sin[\vartheta]}{a^2 + r^2}$$



$$\tilde{\mathbb{N}} = q_a \hat{N}^a$$


In[180]:= Nt = Sum[NhA[[ii + 1]] × qa[[ii]], {ii, 1, 2}] // Simplify
Ntbar = Nt /. J → -J;


$$\frac{2 a J M r (a^2 + 2 r^2 + a^2 \cos[2 \vartheta]) \sin[\vartheta]}{(a^2 + r^2) (a^4 + 2 r^4 + a^2 r (2 M + 3 r) + a^2 (a^2 + r (-2 M + 3 r)) \cos[2 \vartheta])}$$

```

Asymptotic behaviour of  $\mathbb{N}$  and  $\tilde{\mathbb{N}}$  is compatible with the derived fall-off conditions

```
In[178]:= Series[N, {r, ∞, 3}]
Series[Nt, {r, ∞, 3}]


$$\frac{2 a J M \sin[\vartheta]}{r} - \frac{2 (a^3 J M \sin[\vartheta])}{r^3} + O\left[\frac{1}{r}\right]^4$$



$$\frac{2 a J M \sin[\vartheta]}{r^3} + O\left[\frac{1}{r}\right]^4$$



$$\mathbf{a} = \frac{1}{2} \hat{\gamma}_{ab} q^a \bar{q}^b$$


In[187]:= a =  $\frac{1}{2}$  Sum[yhab[[ii, jj]] × qA[[ii]] × qbA[[jj]], {ii, 1, 2}, {jj, 1, 2}] /. J^2 → -1 // Simplify


$$\frac{3 a^4 + 8 r^4 + 2 a^2 r (2 M + 5 r) + 2 a^2 (2 a^2 + r (-2 M + 3 r)) \cos[2 \vartheta] + a^4 \cos[2 \vartheta]^2}{4 (a^2 + 2 r^2 + a^2 \cos[2 \vartheta])}$$



$$\mathbf{b} = \frac{1}{2} \hat{\gamma}_{ab} q^a q^b$$


In[188]:= b =  $\frac{1}{2}$  Sum[yhab[[ii, jj]] × qA[[ii]] × qA[[jj]], {ii, 1, 2}, {jj, 1, 2}] /. J^2 → -1 // Simplify
bbar = b /. J → -J;


$$- \frac{a^2 (a^2 + 2 r (2 M + r) + a^2 \cos[2 \vartheta]) \sin[\vartheta]^2}{2 (a^2 + 2 r^2 + a^2 \cos[2 \vartheta])}$$

```

Asymptotic behaviour of  $\mathfrak{a}$  and  $\mathfrak{b}$  is compatible with the derived fall-off conditions

```
In[194]:= Series[\mathfrak{a}, {r, \infty, 0}]
Series[\mathfrak{b}, {r, \infty, 0}]

Out[194]= r^2 + \frac{1}{4} \times (3 a^2 + a^2 \text{Cos}[2 \vartheta]) + O\left[\frac{1}{r}\right]^1

Out[195]= -\frac{1}{2} a^2 \text{Sin}[\vartheta]^2 + O\left[\frac{1}{r}\right]^1

In[196]:= \mathfrak{d} = \mathfrak{a}^2 - \mathfrak{b} \mathfrak{bbar} // Simplify

Out[196]= \frac{1}{2} (a^4 + 2 r^4 + a^2 r (2 M + 3 r) + a^2 (a^2 + r (-2 M + r)) \text{Cos}[2 \vartheta])

\hat{\gamma}_{ab} = \mathfrak{a} q_{ab} + \frac{1}{2} [\bar{\mathfrak{b}} q_a q_b + \mathfrak{b} \bar{q}_a \bar{q}_b]

In[197]:= CHECK == \gamma_{hab} - \left( \frac{\mathfrak{a}}{2} \text{Table}[\mathfrak{qa}[\mathfrak{i}] \times \mathfrak{qba}[\mathfrak{j}] + \mathfrak{qba}[\mathfrak{i}] \times \mathfrak{qa}[\mathfrak{j}], \{\mathfrak{i}, 1, 2\}, \{\mathfrak{j}, 1, 2\}] + \right.
\frac{1}{2} \text{Table}[\mathfrak{bbar} \mathfrak{qa}[\mathfrak{i}] \times \mathfrak{qa}[\mathfrak{j}] + \mathfrak{b} \mathfrak{qba}[\mathfrak{i}] \times \mathfrak{qba}[\mathfrak{j}], \{\mathfrak{i}, 1, 2\}, \{\mathfrak{j}, 1, 2\}]) \Big) /. J^2 \rightarrow -1 // Simplify

Out[197]= CHECK == {{0, 0}, {0, 0}}

\hat{\gamma}^{ab} = \mathfrak{d}^{-1} \left\{ \mathfrak{a} q^{ab} - \frac{1}{2} [\bar{\mathfrak{b}} q^a q^b + \mathfrak{b} \bar{q}^a \bar{q}^b] \right\}

In[198]:= CHECK == \gamma^{hab} - \left( \mathfrak{d}^{-1} \left( \frac{\mathfrak{a}}{2} \text{Table}[\mathfrak{qA}[\mathfrak{i}] \times \mathfrak{qbA}[\mathfrak{j}] + \mathfrak{qbA}[\mathfrak{i}] \times \mathfrak{qA}[\mathfrak{j}], \{\mathfrak{i}, 1, 2\}, \{\mathfrak{j}, 1, 2\}] - \right. \right.
\frac{1}{2} \text{Table}[\mathfrak{bbar} \mathfrak{qA}[\mathfrak{i}] \times \mathfrak{qA}[\mathfrak{j}] + \mathfrak{b} \mathfrak{qbA}[\mathfrak{i}] \times \mathfrak{qbA}[\mathfrak{j}], \{\mathfrak{i}, 1, 2\}, \{\mathfrak{j}, 1, 2\}]) \Big) \Big) /. J^2 \rightarrow -1 // Simplify

Out[198]= CHECK == {{0, 0}, {0, 0}}

\hat{N}_a = \frac{1}{2} (\bar{\mathfrak{N}} q_a + \mathfrak{N} \bar{q}_a)

In[199]:= CHECK == N_{ha} - \left( \frac{\mathfrak{Nbar}}{2} \mathfrak{qa} + \frac{\mathfrak{N}}{2} \mathfrak{qba} \right) /. J^2 \rightarrow -1 // Simplify

Out[199]= CHECK == {0, 0}

\hat{N}^a = \frac{1}{2} (\tilde{\mathfrak{N}} q^a + \tilde{\mathfrak{N}} \bar{q}^a)

In[200]:= CHECK == Table[N_{ha}[\mathfrak{i} + 1], \{\mathfrak{i}, 1, 2\}] - \left( \frac{\mathfrak{Ntbar}}{2} \mathfrak{qA} + \frac{\mathfrak{Nt}}{2} \mathfrak{qbA} \right) /. J^2 \rightarrow -1 // Simplify

Out[200]= CHECK == {0, 0}

In[201]:= CHECK == \mathfrak{Nt} - \mathfrak{d}^{-1} (\mathfrak{a} \mathfrak{N} - \mathfrak{b} \mathfrak{Nbar}) // Simplify

Out[201]= CHECK == 0
```

## ■ Extrinsic curvature

$K_{ab}$  is decomposed into  $\kappa$ ,  $k_a$ ,  $\mathbf{K}$  and  $\mathring{K}_{ab}$ .  $\kappa$  and  $\mathbf{K}$  are spin-weight 0 functions but we have to take the spin-weight 1  $\mathbf{k} = q^a k_a$  component and spin-weight 2  $\mathring{\mathbf{K}}_{qq} = q^a q^b \mathring{K}_{ab}$  component.

Asymptotic behaviour of  $\kappa$  and  $\mathbf{K}$  is in accordance with the derived fall-off conditions

```
In[204]:= Series[\kappa, {r, \infty, 3}]
Series[\mathbf{K}, {r, \infty, 3}]

Out[204]= \frac{2 M}{r^2} - \frac{4 M^2}{r^3} + O\left[\frac{1}{r}\right]^4

Out[205]= -\frac{4 M}{r^2} + \frac{4 M^2}{r^3} + O\left[\frac{1}{r}\right]^4

\mathbf{k} = k_a q^a

In[206]:= \mathbf{k} = \text{Sum}[\mathfrak{kka}[\mathfrak{ii}] \times \mathfrak{qA}[\mathfrak{ii}], \{\mathfrak{ii}, 1, 2\}] // Simplify
\mathbf{kbar} = \mathbf{k} /. J \rightarrow -J;

2 a M \left( -J (a^4 - 3 a^2 r^2 - 6 r^4 + a^2 (a^2 - r^2) \text{Cos}[2 \vartheta]) \text{Sin}[\vartheta] + \frac{a r (a^2 + 2 r^2 + a^2 \text{Cos}[2 \vartheta])^2 \text{Sin}[2 \vartheta]}{a^2 + 2 r (2 M + r) + a^2 \text{Cos}[2 \vartheta]} \right)

Out[206]= \frac{\sqrt{\frac{2 M r + r^2 + a^2 \text{Cos}[\vartheta]^2}{2 r^2 + 2 a^2 \text{Cos}[\vartheta]^2}} (a^2 + 2 r^2 + a^2 \text{Cos}[2 \vartheta])^3 \sqrt{\frac{a^4 + 2 r^4 + a^2 r (2 M + 3 r) + a^2 (a^2 + r (-2 M + r)) \text{Cos}[2 \vartheta]}{(a^2 + 2 r^2 + a^2 \text{Cos}[2 \vartheta]) (a^2 + 2 r (2 M + r) + a^2 \text{Cos}[2 \vartheta])}}}{1}

\mathring{\mathbf{K}}_{qq} = \mathring{\mathbf{K}}_{ab} q^a q^b \text{ and } \mathring{\mathbf{K}}_{q\bar{q}} = \mathring{\mathbf{K}}_{ab} q^a \bar{q}^b
```

In[209]:= **Kcqq = Sum[qA[[i,i]] \* qA[[j,j]] \* KKcab[[i,i],j,j]],{i,i,1,2},{j,j,1,2}]/.J^2 -> -1 // Simplify**  
**Kcqqlbar = Kcqq /. J -> -J;**  
**Kcqqlb = Sum[qA[[i,i]] \* qbA[[j,j]] \* KKcab[[i,i],j,j]],{i,i,1,2},{j,j,1,2}]/.J^2 -> -1 // Simplify**

Out[209]= 
$$\frac{a^2 M r \left( \frac{16 a J \cos[\vartheta]}{(a^2+2 r^2+a^2 \cos[2 \vartheta])^2} + \frac{4 a^2 (M-r)-8 r^2 (3 M+r)+4 a^2 (M-r) \cos[2 \vartheta]}{(a^2+2 r^2+a^2 \cos[2 \vartheta])^3} + \frac{a^2 (M-r)-2 r^2 (3 M+r)+a^2 (M-r) \cos[2 \vartheta]}{(r^2+a^2 \cos[\vartheta]^2) (a^4+2 r^4+a^2 r (2 M+3 r)+a^2 (a^2+r (-2 M+r)) \cos[2 \vartheta])} \right) \sin[\vartheta]^2}{\sqrt{1+\frac{2 M r}{r^2+a^2 \cos[\vartheta]^2}}}$$

Out[211]= 
$$-\frac{4 a^4 M r (a^2+2 r (2 M+r)+a^2 \cos[2 \vartheta]) (a^2 (M-r)-2 r^2 (3 M+r)+a^2 (M-r) \cos[2 \vartheta]) \sin[\vartheta]^4}{\sqrt{1+\frac{2 M r}{r^2+a^2 \cos[\vartheta]^2}} (a^2+2 r^2+a^2 \cos[2 \vartheta])^3 (a^4+2 r^4+a^2 r (2 M+3 r)+a^2 (a^2+r (-2 M+r)) \cos[2 \vartheta])}$$

Asymptotic behaviour of  $k$  and  $\overset{\circ}{K}_{qq}$  is better than expected from the fall-off conditions

In[213]:= **Series[k,{r,Infinity,3}]**  
**Series[Kcqq,{r,Infinity,3}]**

Out[213]= 
$$\frac{3 a J M \sin[\vartheta]}{r^2} + \frac{a^2 M \sin[2 \vartheta]}{r^3} + O\left[\frac{1}{r}\right]^4$$

Out[214]= 
$$-\frac{2 (a^2 M \sin[\vartheta]^2)}{r^2} + \frac{a^2 M (-4 M+4 a J \cos[\vartheta]) \sin[\vartheta]^2}{r^3} + O\left[\frac{1}{r}\right]^4$$

In[215]:= **CHECK == Kcqqlb - \frac{1}{2 a} (b Kcqqlbar + bbar Kcqq) /. J^2 -> -1 // Simplify**

Out[215]= CHECK == 0

In[216]:= **CHECK == (kka - (\frac{k}{2} qba + \frac{kbar}{2} qa) // Simplify) /. J^2 -> -1**

Out[216]= CHECK == {0, 0}

In[217]:= **CHECK == (KKcab - (\frac{1}{4} Kcqqlb Table[qa[[i]] \* qbA[[j]] + qa[[j]] \* qbA[[i]],{i,1,2},{j,1,2}] + \frac{1}{4} Table[Kcqqlbar qa[[i]] \* qa[[j]] + Kcqq qbA[[i]] \* qbA[[j]],{i,1,2},{j,1,2}]) // Simplify) /. J^4 -> 1 /. J^2 -> -1**

Out[217]= CHECK == {{0, 0}, {0, 0}}

■ Secondary extrinsic curvature

$\hat{K}_{qq} = \hat{K}_{ab} q^a q^b$  and  $\hat{K}_{q\bar{q}} = \hat{K}_{ab} q^a \bar{q}^b$

These variables could be computed from other, more basic variables determined earlier (see next section)

In[218]:= **Khqq = Sum[qA[[i,i]] \* qA[[j,j]] \* Khab[[i,i],j,j]],{i,i,1,2},{j,j,1,2}]/.J^2 -> -1 // Simplify**  
**Khqqqlbar = Khqq /. J -> -J;**  
**Khqqqlb = Sum[qA[[i,i]] \* qbA[[j,j]] \* Khab[[i,i],j,j]],{i,i,1,2},{j,j,1,2}]/.J^2 -> -1 // Simplify**

Out[218]= 
$$-\left( \sqrt{2} a^2 M (3 a^6+2 a^4 M r+3 a^4 r^2-8 a^2 M r^3-8 a^2 r^4-8 r^6+16 a J M r^2 (3 a^2+4 r^2) \cos[\vartheta]+4 a^2 (a^4+a^2 r^2+2 M r^3) \cos[2 \vartheta]+16 a^3 J M r^2 \cos[3 \vartheta]+a^6 \cos[4 \vartheta]-2 a^4 M r \cos[4 \vartheta]+a^4 r^2 \cos[4 \vartheta]) \sin[\vartheta]^2 \right) / \left( (a^2+2 r^2+a^2 \cos[2 \vartheta])^3 (a^2+2 r (2 M+r)+a^2 \cos[2 \vartheta]) \sqrt{\frac{a^4+2 r^4+a^2 r (2 M+3 r)+a^2 (a^2+r (-2 M+r)) \cos[2 \vartheta]}{(a^2+2 r^2+a^2 \cos[2 \vartheta]) (a^2+2 r (2 M+r)+a^2 \cos[2 \vartheta])}} \right)$$

Out[220]= 
$$\frac{\frac{4 M^2 r^3}{(r^2+a^2 \cos[\vartheta]^2) (r (2 M+r)+a^2 \cos[\vartheta]^2)} + \frac{2 r (a^2+r (-2 M+r))}{a^2+2 r^2+a^2 \cos[2 \vartheta]}}{\sqrt{\frac{4 M^2 r^2}{(r^2+a^2 \cos[\vartheta]^2) (r (2 M+r)+a^2 \cos[\vartheta]^2)} + \frac{2 (a^2+r (-2 M+r))}{a^2+2 r^2+a^2 \cos[2 \vartheta]}}} + \frac{(a^4+2 r^4+a^2 r (2 M+3 r)+a^2 (a^2+r (-2 M+r)) \cos[2 \vartheta]) (a^4 M+3 a^4 r-4 a^2 M r^2+8 a^2 r^3+8 r^5+4 a^2 r (a^2+r (M+2 r)) \cos[2 \vartheta]-a^4 (M-r) \cos[4 \vartheta])}{(a^2+2 r^2+a^2 \cos[2 \vartheta])^3 (a^2+2 r (2 M+r)+a^2 \cos[2 \vartheta]) \sqrt{\frac{4 M^2 r^2}{(r^2+a^2 \cos[\vartheta]^2) (r (2 M+r)+a^2 \cos[\vartheta]^2)} + \frac{2 (a^2+r (-2 M+r))}{a^2+2 r^2+a^2 \cos[2 \vartheta]}}}$$

■ Derived quantities

This section is to quantities that could be derived from the basic  $a, b, R(=2), \hat{N}, N, k, K, \overset{\circ}{K}_{qq}$  and  $\kappa$  variables.

The action of the covariant derivative operator compatible with the unit sphere metric on the metric induced on the 2-surfaces,  $\overset{\circ}{D}_a \hat{Y}_{bc}$

In[222]:= **Dyhabc = Table[D[yhab[[j,k]],zA[[i]]]-Sum[GammaQabc[[i,i],j]] \* yhab[[i,i],k],{i,i,1,2}]-Sum[GammaQabc[[i,i],i,k]] \* yhab[[i,i],j],{i,i,1,2}],{i,1,2},{j,1,2},{k,1,2}] // Simplify;**

Connection relating the covariant derivative operators compatible with  $q_{ab}$  and  $\hat{Y}_{ab}$

In[223]:= **CABC = Table[Sum[\frac{yhab[[i,i]]}{2} (Dyhabc[[j,ii,k]]+Dyhabc[[k,j,ii]]-Dyhabc[[ii,j,k]]),{ii,1,2}],{i,1,2},{j,1,2},{k,1,2}] // Simplify;**

Components of the connection

```
In[224]:= A = Sum[qA[i i] * qA[j j] * qba[k k] * CAbc[k k, i i, j j], {i i, 1, 2}, {j j, 1, 2}, {k k, 1, 2}] /. J^2 -> -1 // Simplify
A2 = d^-1 (a (2 d[a, 0] - D[b, 2]) - bbar d[b, 2]);
CHECK == A - A2 // Simplify
Abar = A /. J -> -J;
```

$$\frac{1}{(a^2 + 2 r^2 + a^2 \cos[2 \vartheta])^3} a^2 \left( -\frac{16 M r (a^2 + r^2) \cos[\vartheta] (a^2 + 2 r^2 + a^2 \cos[2 \vartheta])^2 \sin[\vartheta]}{a^4 + 2 r^4 + a^2 r (2 M + 3 r) + a^2 (a^2 + r (-2 M + r)) \cos[2 \vartheta]} - \right. \\ \left. \cos[\vartheta] (3 a^4 + 24 a^2 M r + 8 a^2 r^2 + 32 M r^3 + 8 r^4 + 4 a^2 (a^2 + 2 r (M + r)) \cos[2 \vartheta] + a^4 \cos[4 \vartheta]) \sin[\vartheta] + (a^2 + 2 r^2 + a^2 \cos[2 \vartheta])^2 \sin[2 \vartheta] \right)$$

```
Out[226]= CHECK == 0
```

```
In[228]:= B = Sum[qbA[i i] * qA[j j] * qa[k k] * CAbc[k k, i i, j j], {i i, 1, 2}, {j j, 1, 2}, {k k, 1, 2}] /. J^2 -> -1 // Simplify
B2 = d^-1 (a D[b, 2] - b d[bbar, -2]);
CHECK == B - B2 // Simplify
Bbar = B /. J -> -J;
```

$$\frac{a^2 (3 a^4 + 12 a^2 M r + 8 a^2 r^2 + 16 M r^3 + 8 r^4 + 4 a^2 (a^2 + r (M + 2 r)) \cos[2 \vartheta] + a^4 \cos[4 \vartheta]) \sin[2 \vartheta]}{(a^2 + 2 r^2 + a^2 \cos[2 \vartheta])^3}$$

```
Out[230]= CHECK == 0
```

```
In[232]:= C = Sum[qA[i i] * qA[j j] * qa[k k] * CAbc[k k, i i, j j], {i i, 1, 2}, {j j, 1, 2}, {k k, 1, 2}] /. J^2 -> -1 // Simplify
C2 = d^-1 (a d[b, 2] - b (2 d[a, 0] - D[b, 2]));
CHECK == C - C2 // Simplify
Cbar = C /. J -> -J;
```

$$-\frac{16 a^4 M r \cos[\vartheta] (a^4 + 3 a^2 r (2 M + r) + 2 r^3 (4 M + r) + a^2 (a^2 + r (2 M + r)) \cos[2 \vartheta]) \sin[\vartheta]^3}{(a^2 + 2 r^2 + a^2 \cos[2 \vartheta])^3 (a^4 + 2 r^4 + a^2 r (2 M + 3 r) + a^2 (a^2 + r (-2 M + r)) \cos[2 \vartheta])}$$

```
Out[234]= CHECK == 0
```

$$K_{ab}^* = \hat{K}_{ab} \hat{N}$$

```
In[236]:= KKstar = Khat Nh;
```

```
In[237]:= CHECK == KKstar - ((a (D[a, r] - D[N, 1] + Bbar N) - b (D[bbar, r] - D[Nbar, -1] + Cbar N / 2 + Abar Nbar)) / (2 d) + \\ (a (D[a, r] - d[Nbar, -1] + B Nbar) - bbar (D[b, r] - d[N, 1] + C Nbar / 2 + A N)) / (2 d)) // Simplify
```

```
Out[237]= CHECK == 0
```

```
In[238]:= KKstarqq = Khqq Nh;
```

```
In[239]:= KKstarqqb = Khqqb Nh;
```

```
In[240]:= LieKhat = Sum[nhA[i i] * D[Khat, yA[i i]], {i i, 1, 3}];
```

```
In[241]:= RyhabcD = Table[-D[GammaAbc[l, j, k], zA[i i]] + D[GammaAbc[l, i, k], zA[j j]] + \\ Sum[-GammaAbc[l, i, i i] * GammaAbc[i i, j, k] + GammaAbc[l, j, i i] * GammaAbc[i i, i, k], {i i, 1, 2}], {i, 1, 2}, {j, 1, 2}, {k, 1, 2}, {l, 1, 2}];
Ryhab = Table[Sum[RyhabcD[i, i i, j, i i], {i i, 1, 2}], {i, 1, 2}, {j, 1, 2}];
Ryh = Simplify[Sum[Ryhab[i i, j j] * yhAB[i i, j j], {i i, 1, 2}, {j j, 1, 2}]];
```

```
In[244]:= KcKc = Sum[KKcab[i i, j j] * KKcAB[i i, j j], {i i, 1, 2}, {j j, 1, 2}];
```

```
In[245]:= KhKh = Sum[Khab[i i, j j] * KhAB[i i, j j], {i i, 1, 2}, {j j, 1, 2}];
```

```
In[246]:= KsKs = KhKh Nh Nh;
```

```
In[247]:= KcKs = Nh Sum[KKcab[i i, j j] * KhAB[i i, j j], {i i, 1, 2}, {j j, 1, 2}];
```

```
In[248]:= yh = Sqrt[Det[yhab]];
```

```
In[249]:= DhDhNh = 1/yh Sum[D[yh Sum[yhAB[i i, j j] * D[Nh, zA[j j]], {j j, 1, 2}], zA[i i], {i i, 1, 2}];
```

```
DhDhNh2 = Sum[yhAB[i i, j j] * (D[Nh, zA[i i], zA[j j]] - Sum[GammaAbc[k k, i i, j j] * D[Nh, zA[k k]], {k k, 1, 2}]), {i i, 1, 2}, {j j, 1, 2}];
CHECK == DhDhNh - DhDhNh2 // Simplify
```

```
Out[251]= CHECK == 0
```

```
In[252]:= RhabcD = Table[-D[GammaAbc[l, j, k], yA[i i]] + D[GammaAbc[l, i, k], yA[j j]] + \\ Sum[-GammaAbc[l, i, i i] * GammaAbc[i i, j, k] + GammaAbc[l, j, i i] * GammaAbc[i i, i, k], {i i, 1, 3}], {i, 1, 3}, {j, 1, 3}, {k, 1, 3}, {l, 1, 3}];
Rhab = Table[Sum[RhabcD[i, i i, j, i i], {i i, 1, 3}], {i, 1, 3}, {j, 1, 3}];
Rh = Simplify[Sum[Rhab[i i, j j] * hAB[i i, j j], {i i, 1, 3}, {j j, 1, 3}]];
```

```
CHECK == Simplify[(% /. a -> 0) - (8 M^2 / (r^4 (1 + 2 M / r)^2))]
```

```
Out[255]= CHECK == 0
```

```
In[256]:= kappa0 = Rh - KcKc;
```

## ■ Algebraic-hyperbolic system

```

In[257]:= KcKh = Sum[KKcAB[[i, j]] * Kh2ab[[i, j]], {i, 1, 2}, {j, 1, 2}];

In[258]:= F = 
$$\frac{N_h}{4 d} (2 a B \bar{k} - b (C \bar{k} + A \bar{k}) + 2 a B \bar{k} - b \bar{b} (C \bar{k} + A \bar{k})) - \frac{1}{d} ((a \bar{k} - b \bar{k}) \delta[N_h, 0] + (a \bar{k} - b \bar{k}) \mathcal{D}[N_h, 0] + N_h (KcKh - (\kappa \kappa - KK / 2) \text{Khat})) -$$


In[259]:= RHSK = 
$$\frac{N_t}{2} \mathcal{D}[KK, 0] + \frac{N_{tbar}}{2} \delta[KK, 0] + \frac{N_h}{2 d} (a (\delta[\bar{k}, -1] + \mathcal{D}[\bar{k}, 1]) - b \mathcal{D}[\bar{k}, -1] - \bar{b} \delta[\bar{k}, 1]) - F;$$


In[260]:= RHSKT1 = 
$$\frac{N_t}{2} \mathcal{D}[KK, 0] + \frac{N_{tbar}}{2} \delta[KK, 0] + \frac{N_h}{2 d} (a (\delta[\bar{k}, -1] + \mathcal{D}[\bar{k}, 1]) - b \mathcal{D}[\bar{k}, -1] - \bar{b} \delta[\bar{k}, 1]);$$


In[261]:= CHECK == D[KK, r] - RHSK /. a -> 1/2 /. M -> 1 /. phi -> pi/2 // Simplify
CHECK == D[KK, r] - RHSK /. a -> 1/2 /. M -> 1 /. phi -> 2 pi/3 // Simplify
CHECK == D[KK, r] - RHSK /. a -> 2/3 /. M -> 1 /. phi -> 2 pi/3 // Simplify
CHECK == D[KK, r] - RHSK /. a -> 1/2 /. M -> 3 /. phi -> 2 pi/3 // Simplify

Out[261]= CHECK == 0

Out[262]= CHECK == 0

Out[263]= CHECK == 0

Out[264]= CHECK == 0

In[275]:= dotnhatA2 = Table[-Sum[yhAB[[i, i]] * D[Log[Nh], zA[[i]]], {i, 1, 2}], {i, 1, 2}];
DhKKca = Table[Sum[yhAB[[i, j]] * (D[KKcab[[j, i]], zA[[i]] - Sum[GyhAbc[[kk, i, j]] * KKcab[[kk, i]], {kk, 1, 2}) - Sum[GyhAbc[[kk, i, j]] * KKcab[[kk, i]], {kk, 1, 2})), {i, 1, 2}, {j, 1, 2}], {i, 1, 2}];
dotnhatKKca = Table[Sum[dotnhatA2[[i]] * KKcab[[i, i]], {i, 1, 2}], {i, 1, 2}];

In[268]:= NqnKc = Nh Sum[qA[[i]] * dotnhatKKca[[i]], {i, 1, 2}];

In[271]:= NqDKc = Sum[qA[[i]] * DhKKca[[i]], {i, 1, 2}];

In[278]:= f = 
$$-\frac{1}{2} (\bar{k} \delta[N_{tbar}, -1] + \bar{k} \delta[N_t, 1]) + \frac{N_h}{2 d KK} ((a \bar{k} - b \bar{k}) (B \bar{k} + B \bar{k}) + (a \bar{k} - b \bar{k}) (C \bar{k} + A \bar{k})) - (\kappa \kappa - KK / 2) \delta[N_h, 0] + N_h \left( \frac{\delta[\kappa 0, 0]}{2 KK} + \text{Khat } \bar{k} - \text{Sum}[qA[[i]] * \text{dotnhatKKca}[[i]], \{i, 1, 2\}] + \text{Sum}[qA[[i]] * DhKKca[[i]], \{i, 1, 2\}] \right);$$


In[279]:= RHSk = 
$$\frac{N_t}{2} \mathcal{D}[\bar{k}, 1] + \frac{N_{tbar}}{2} \delta[\bar{k}, 1] - \frac{N_h}{KK} \left( \kappa \delta[KK, 0] - \frac{(a \bar{k} - b \bar{k}) \delta[\bar{k}, -1] + (a \bar{k} - b \bar{k}) \delta[\bar{k}, 1]}{d} \right) - f;$$


In[280]:= RHSKT1 = 
$$\frac{N_t}{2} \mathcal{D}[\bar{k}, 1] + \frac{N_{tbar}}{2} \delta[\bar{k}, 1] - \frac{N_h}{KK} \left( \kappa \delta[KK, 0] - \frac{(a \bar{k} - b \bar{k}) \delta[\bar{k}, -1] + (a \bar{k} - b \bar{k}) \delta[\bar{k}, 1]}{d} \right);$$


In[281]:= CHECK == D[k, r] - RHSk /. a -> 1/2 /. M -> 1 /. phi -> pi/2 // Simplify
CHECK == Simplify[D[k, r] - RHSk /. a -> 1/2 /. M -> 1 /. phi -> 2 pi/3] /. J^2 -> -1
CHECK == Simplify[D[k, r] - RHSk /. a -> 2/3 /. M -> 1 /. phi -> 2 pi/3] /. J^2 -> -1
CHECK == Simplify[D[k, r] - RHSk /. a -> 1/2 /. M -> 3 /. phi -> 2 pi/3] /. J^2 -> -1

Out[281]= CHECK == 0

Out[282]= CHECK == 0

Out[283]= CHECK == 0

Out[284]= CHECK == 0

In[285]:= kappaT1 = 
$$\frac{2 \text{Sum}[kkA[[i]] * kka[[i]], \{i, 1, 2\}] - \kappa 0}{2 KK};$$


In[286]:= kappaT2 = Sum[kkA[[i]] * kka[[i]], {i, 1, 2}];

In[287]:= kappaT2 - ((2 a k kbar - b kbar kbar - bbar k k) / (2 d)) /. J -> i // Simplify

Out[287]= 0

In[288]:= CHECK == 
$$\kappa \kappa - \left( \frac{2 \text{Sum}[kkA[[i]] * kka[[i]], \{i, 1, 2\}] - KK^2 / 2 - \kappa 0}{2 KK} \right) /. \phi \rightarrow \pi/2 // FullSimplify$$


CHECK == 
$$\kappa \kappa - \left( \frac{2 \text{Sum}[kkA[[i]] * kka[[i]], \{i, 1, 2\}] - KK^2 / 2 - \kappa 0}{2 KK} \right) /. \phi \rightarrow \pi/3 // FullSimplify$$


CHECK == 
$$\kappa \kappa - \left( \frac{2 \text{Sum}[kkA[[i]] * kka[[i]], \{i, 1, 2\}] - KK^2 / 2 - \kappa 0}{2 KK} \right) /. \phi \rightarrow \pi/6 // FullSimplify$$


Out[288]= CHECK == 0

Out[289]= CHECK == 0

Out[290]= CHECK == 0

```
